# Supplementary material for: Individuals, Institutions, and Innovation in the Debates of the French Revolution
Source: arXiv:1710.06867 ancillary file (2017-10-18)
Supplement: Supplementary file 1 [file supplementary_information.pdf]

# Supplementary Information for Individuals, Institutions, and Innovation in the Debates of the French Revolution

Alexander T. J. Barron, Jenny Huang, Rebecca L. Spang, Simon DeDeo

## Contents

**1 Preparing and characterizing speech data** **1**
1.1 Data preparation . . . . . . . . . . . . . . . . . . . . . . . . . . . 1

**2 Novelty, transience, and resonance** **8**
2.1 Presidential speech removal . . . . . . . . . . . . . . . . . . . . . . 9
2.2 Novelty, transience, and resonance over time . . . . . . . . . . . . 10

**3 Role behavior** **10**

**4 Defining committee speech** **12**
4.1 Committee speech and information processing . . . . . . . . . . . 15

**5 Synchronic modeling of role behavior** **16**
5.1 Consistency of measurements over multiple timescales . . . . . . 18

**6 Diachronic modeling of role behavior** **20**
6.1 Single epoch model . . . . . . . . . . . . . . . . . . . . . . . . . . 20
6.2 Two-epoch models . . . . . . . . . . . . . . . . . . . . . . . . . . 20
6.3 Explaining the time dependence in the single-epoch model . . . . 24
6.4 Two-epoch model with fixed intercept . . . . . . . . . . . . . . . 25
6.5 Including all roles in the two-epoch model . . . . . . . . . . . . . 25

**7 Topic modeling** **49**

## 1. Preparing and characterizing speech data

### *1.1. Data preparation*

We create our corpus from the Archives Parlementaires (AP) of the French Revolution Digital Archive (FRDA), a digitized collection of texts made available through the efforts of Stanford University Libraries and the Bibliothéque nationale de France. These texts, which span the years 1787-1794, include transcripts of parliamentary deliberations, letters, reports, speeches, court actions, and other first-hand accounts of the proceedings of the National Assembly, National Constituent Assembly, and Legislative Assembly.

FRDA files use Text Encoding Initiative (TEI) guidelines, so tag structure is consistent and produces valid xml. The TEI structure follows the formatting of

the original document, tracking individual speeches. For example, the following rhetorical exchange:

```
<sp>
  <speaker>M. de Menou.</speaker>
  <p> Je demande qu'on n'interrompe pas M. l'abbé Maury. En parlant contre
  la chose publique, il lui fait plus de bien que ceux qui parlent pour.
  </p>
</sp>
<sp>
  <speaker>M. l'abbé Maury.</speaker>
  <p> Pour continuerà servir la chose publique, j'examinerai quels ont
  été les résultats de cette usurpation d'autorité de la part de votre
  comit\'{e} ecclésiastique. (On rappelle M. l'abbé Maury à l'ordre). M. de
  Mirabeau a parlé dans cette discussion et a renforcé de sa théologie les
  arguments qui nous avaient déjà été présentés. A Dieu ne plaise que je
  veuille rapprocher ici les principes qu'il a posés en faveur de la
  religion avec les conséquences qu'il en a tirées. Il ne nous est permis
  de scruter les intentions de personne. M. de Mirabeau vous a dit que les
  évêques devaient se faire d'autant moins de scrupules d'outrepasser les
  circonscriptions actuelles de leurs diocèses que chaque évêque était un
  évêque universel, que sa juridiction était reconnue par les canons, et
  que c'était le premier des quatre articles enseignés par le clergé de
  France en 1682. Cela est trop important, trop capable de faire illusion
  pour que je ne rappelle pas ici la vérité ; je ne calomnie pas les
  intentions de M. de Mirabeau.... Je rapporte ses propres expressions.
  </p>
</sp>
<sp>
  <speaker>M. de Mirabeau.</speaker>
  <p>Non!</p>
</sp>
<sp>
  <speaker>M. l'abbé Maury.</speaker>
  <p>Il m'est extrêmement important de savoir ce que M. de Mirabeau a dit.</p>
</sp>
<sp>
  <speaker>M. de Mirabeau.</speaker>
  <p>Permettez, monsieur....</p>
</sp>
<sp>
  <speaker>M. l'abbé Maury.</speaker>
  <p>Je prends la liberté de demander publiquement à M. de Mirabeau s'il
  n'a pas dit que tout évêque était un évêque universel? si je me suis
  trompé je vais être redressé.</p>
</sp>
<sp>
  <speaker>M. dé Mirabeau.</speaker>
  <p>Je réponds, monsieur, que je n'ai jamais dit que tout évêque fait un
  évêque</p>
  <p>universel ; ces ridicules paroles ne sont jamais sorties que de votre
  bouche. J'ai dit que, suivant le premier des quatre articles des
  libertés de l'Eglise gallicane, les évêques recevaient leurs
  juridictions immédiates de Dieu, que l'essence d'un caractère divin
  était de n'être circonscrit par aucune limite et par conséquent d'être
  universel; qu'il me paraissait qu'en toute langue conforme aux règles du
  bon esprit la circonscription diocésaine était purement temporelle,
  qu'elle ressortissait uniquement de la puissance temporelle, et non de
  ce que vous appelez la puissance ecclésiastique. Voilà, monsieur, ce
  j'ai dit ; mais je n'ai jamais prétendu que l'ordination fait d'un évêque
  un évéque universel (On applaudit.)</p>
</sp>
```

Speeches are contained in speech tags (<sp>) and broken into paragraphs (<p>). Each speech is associated with a speaker string contained in speaker

| rank | word | rank | word | rank | word | rank | word |
|---|---|---|---|---|---|---|---|
| 0 | les | 12 | nous | 24 | avec | 36 | avez |
| 1 | que | 13 | cette | 25 | faire | 37 | doit |
| 2 | des | 14 | aux | 26 | son | 38 | faut |
| 3 | qui | 15 | mais | 27 | ses | 39 | sera |
| 4 | est | 16 | ils | 28 | dont | 40 | était |
| 5 | vous | 17 | leur | 29 | comme | 41 | vos |
| 6 | dans | 18 | être | 30 | votre | 42 | ceux |
| 7 | pour | 19 | sont | 31 | soit | 43 | avoir |
| 8 | une | 20 | ces | 32 | lui | 44 | cet |
| 9 | pas | 21 | ont | 33 | peut | 45 | nos |
| 10 | par | 22 | elle | 34 | leurs | 46 | ainsi |
| 11 | sur | 23 | tous | 35 | donc | 47 | avait |

Table 2: Stop words removed from the corpus, ordered using decreasing probability.

tags (<speaker>). We concatenate all paragraphs from each speech tag into single speeches and set text to lower case. Contractions are separated, and all words with fewer than 3 characters are removed. We remove stop words in Table 2, consisting of pronouns, articles, and other common words from the top 100 most probable words. After removal we use the 10,000 most probable words as a vocabulary. The raw corpus contains 44,953 speeches and 9,930,592 words; the vocabulary corpus contains 44,913 speeches and 4,765,773 words. Figure 4 shows the speech and word count per week over the NCA using the final vocabulary. Interestingly, the week of highest speech count contains the "Flight to Varennes", when the King tried to flee France only to be caught after two days. Figures 5 and 6 show the overall vocabulary speech length distribution, and the mean and variance of speech lengths per week.

We coarse-grain the vocabulary words of each speech into a probability distribution over 100 semantic topics using Latent Dirichlet Allocation (LDA; [3]). We use the implementation found in python package lda (`https://pypi.python.org/pypi/lda/1.0.5`), using collapsed Gibbs sampling with default Dirichlet hyperparameters $\alpha = 0.1$ for topics and $\beta = 0.01$ for words. The most probable words for each speech's resulting topic mixture are shown in the tb opics appendix.

Variations in French naming conventions, recording practice, and OCR error required manual collection of speaker strings from the <speaker> tag of each speech into unified individuals. For every month, we examined the most frequent speaker strings, assigning them to known individuals until at least 80% were covered. Figure 6 shows the fraction of coverage per month. Tables 3 and 4 show the top 40 speakers ranked by raw (non-presidential) speech count. The first includes speeches given on behalf of committees; the latter does not (see the appendix on defining committee speech).

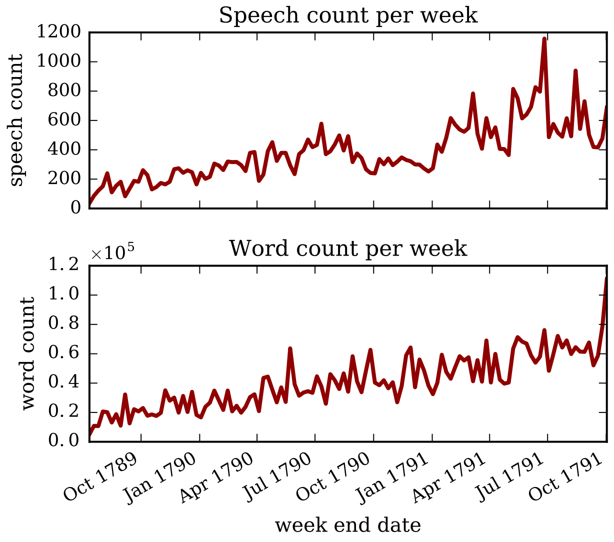


Figure 4: Corpus speech and vocabulary word counts per calendar week. The week of the highest spike in speech count contains the “Flight to Varennes”, when the King and his family attempted to flee France before being caught two days later.

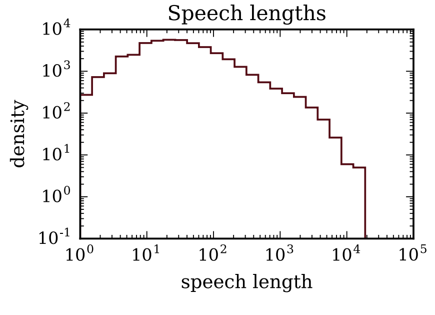


Figure 5: Corpus speech length distribution using our vocabulary.

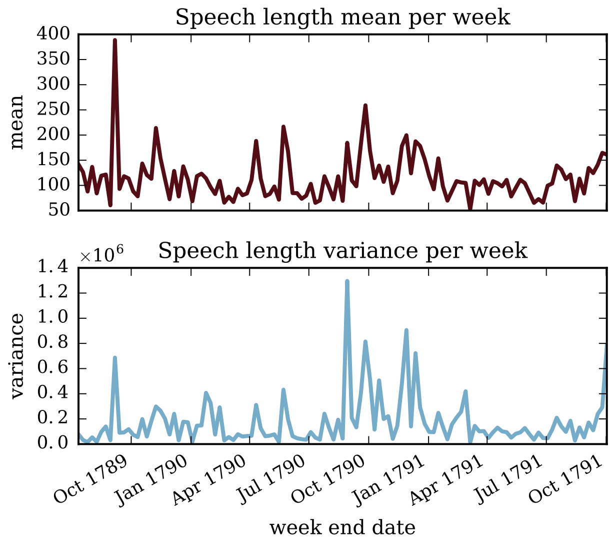


Figure 6: Corpus speech length mean and variance per week.

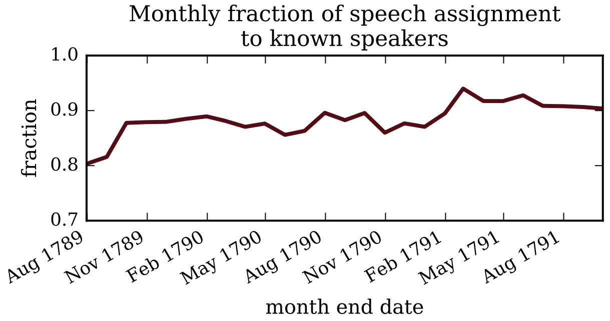


Figure 7: Monthly fraction of speech assignment to known individuals.

| name | rank | speech count |
|---|---|---|
| Jean-Nicolas Desmeunier | 1 | 1027 |
| Armand-Gaston Camus | 2 | 942 |
| Antoine Balthazar Joseph d'Andre | 3 | 864 |
| Isaac René Le Chapelier | 4 | 821 |
| Jean-Sifrein Maury | 5 | 758 |
| Pierre Victor Malouet | 6 | 698 |
| Michel Louis Etienne Regnaud | 7 | 659 |
| Pierre Franąis Bouche | 8 | 653 |
| Jacques Guillaume Thouret | 9 | 636 |
| Honoré Gabriel Riqueti Mirabeau | 10 | 603 |
| Pierre-Louis Prieur de la Marne | 11 | 603 |
| Jacques Antoine Marie de Cazales | 12 | 599 |
| Jean-Denis Lanjuinais | 13 | 596 |
| Louis Simon Martineau | 14 | 595 |
| Adrien Duport | 15 | 522 |
| Antoine Barnave | 16 | 514 |
| Pierre-Louis Roederer | 17 | 494 |
| Jean-Franąis Gaultier de Biauzat | 18 | 470 |
| Emmanuel-Marie-Michel-Philippe Fréteau de Saint Just | 19 | 469 |
| Jean-Franąis Reubell | 20 | 461 |
| Maximilien Robespierre | 21 | 457 |
| Guillaume Franąis Charles Goupil-Préfelne | 22 | 454 |
| Jacques Joseph Defermon de Chapelières | 23 | 449 |
| Antoine Charles Gabriel Folleville | 24 | 415 |
| Philippe-Antoine Merlin | 25 | 399 |
| Jean Baptiste Chabroud | 26 | 384 |
| Charles Malo Franąis Lameth | 27 | 360 |
| Foucauld de Lardimalie | 28 | 335 |
| Jérôme Petion de Villeneuve | 29 | 318 |
| Louis-Michel Le Peletier de Saint-Fargeau | 30 | 303 |
| Franąis Denis Tronchet | 31 | 299 |
| Dominique Garat | 32 | 295 |
| Pierre-Franąis Gossin | 33 | 289 |
| Franąis Dominique de Reynaud Montlosier | 34 | 283 |
| Jean-Louis Emmery | 35 | 269 |
| Théodore Vernier | 36 | 268 |
| Alexandre Lameth | 37 | 264 |
| Charles Antoine Chasset | 38 | 255 |
| Jacques Franąis Menou | 39 | 255 |
| Louis Marie d'Estourmel | 40 | 239 |

Table 3: The top forty identified speakers, ranked by speech count. Presidential speech not included.

| name | rank | speech count |
|---|---|---|
| Antoine Balthazar Joseph d'Andre | 1 | 851 |
| Jean-Sifrein Maury | 2 | 756 |
| Armand-Gaston Camus | 3 | 697 |
| Pierre Victor Malouet | 4 | 684 |
| Michel Louis Etienne Regnaud | 5 | 659 |
| Pierre Franqis Bouche | 6 | 640 |
| Honoré Gabriel Riqueti Mirabeau | 7 | 600 |
| Jacques Antoine Marie de Cazales | 8 | 599 |
| Pierre-Louis Prieur de la Marne | 9 | 595 |
| Louis Simon Martineau | 10 | 541 |
| Isaac René Le Chapelier | 11 | 526 |
| Jean-Denis Lanjuinais | 12 | 490 |
| Antoine Barnave | 13 | 485 |
| Jean-Franqis Reubell | 14 | 461 |
| Jean-Franqis Gaultier de Biauzat | 15 | 461 |
| Maximilien Robespierre | 16 | 457 |
| Guillaume Franqis Charles Goupil-Préfelne | 17 | 450 |
| Emmanuel-Marie-Michel-Philippe Fréteau de Sain... | 18 | 421 |
| Jean-Nicolas Desmeunier | 19 | 417 |
| Antoine Charles Gabriel Folleville | 20 | 414 |
| Pierre-Louis Roederer | 21 | 373 |
| Charles Malo Franqis Lameth | 22 | 358 |
| Jean Baptiste Chabroud | 23 | 351 |
| Adrien Duport | 24 | 337 |
| Foucauld de Lardimalie | 25 | 335 |
| Jérôme Petion de Villeneuve | 26 | 318 |
| Jacques Joseph Defermon de Chapelières | 27 | 304 |
| Dominique Garat | 28 | 294 |
| Philippe-Antoine Merlin | 29 | 289 |
| Franqis Dominique de Reynaud Montlosier | 30 | 283 |
| Franqis Denis Tronchet | 31 | 243 |
| Louis Marie d'Estourmel | 32 | 239 |
| Alexandre Lameth | 33 | 227 |
| Guy Jean Baptiste Target | 34 | 218 |
| Jacques Delavigne | 35 | 206 |
| Bon Albert Briois de Beaumetz | 36 | 205 |
| Jean Louis Gouttes | 37 | 201 |
| Franqis Nicolas Léonard Buzot | 38 | 201 |
| Louis Marie Noailles | 39 | 191 |
| Gislain Louis Bouteville-Dumetz | 40 | 188 |

Table 4: The top forty identified speakers without either presidential or committee speech.

## 2. Novelty, transience, and resonance

We have a list $S$ of speech topic mixtures $s^{(j)} = \left(s_1^{(j)}, s_2^{(j)}, \ldots, s_i^{(j)}, \ldots, s_K^{(j)}\right)$ where $j$ indexes chronological order and $i$ indexes topic, $1 \leq i \leq K$. The novelty of speech $j$ is its mean surprise (KLD) given the speeches within a window of length $w$ beforehand (Figure 8):

$$\mathcal{N}_w(j) = \frac{1}{w} \sum_{d=1}^{w} \mathrm{KLD}\left(s^{(j)} | s^{(j-d)}\right), \tag{4}$$

We refer to $w$ as the measurement scale. Resonance $\mathcal{R}$ is novelty less transience $\mathcal{T}$, where the latter is novelty in Eq. 4 under time reversal:

$$\begin{aligned} \mathcal{R}_w(j) &= \frac{1}{w} \sum_{d=1}^{w} \left[\mathrm{KLD}\left(s^{(j)} | s^{(j-d)}\right) - \mathrm{KLD}\left(s^{(j)} | s^{(j+d)}\right)\right] \\ &= \mathcal{N}_w(j) - \mathcal{T}_w(j) \end{aligned} \tag{5}$$

Novelty and transience are measured relative to a center speech (Figure 8). Figure 1a shows a density plot of novelty and transience per center speech at scale 7. Speeches close to the identity ($x = y$) line are symmetric in surprise from the past and from the future. Resonant speeches break this symmetry, differing more than their past and aligning more with their future. Accordingly, they are found below the identity line where novelty outweighs transience. This asymmetry is evident in Figure 1c, showing box plots of KLDs making up novelty and transience for a sample of resonant center speeches.

Since any speaker is aware of speeches preceding his own, the amount of novelty he displays is under his control. The reception of his speech, as measured by transience, is not. Figure 1a shows our first result using these measures: the riskier one's strategy, the more one is ignored. An increase in novelty is matched in general by an equal increase in transience, shown in the symmetry about the identity line. A speaker might then want to avoid risk altogether, but the real reward lies not in avoiding transience, but maximizing resonance: the power to influence conversation. Using this idea of risk and reward, we measure the expected resonance of any speech given some level of novelty with a linear model:

$$\mathbf{E}[\mathcal{R}|\mathcal{N}] = \beta_{int} + \beta_{\mathcal{N}}\mathcal{N} + \sigma. \tag{6}$$

Figure 1d shows the relationship between resonance and novelty. As shown by the ordinary least squares (OLS) fit line, resonance increases with novelty overall, our second result. The more novel one is, the greater influence over the following speeches one has. We define the rate of this increase as novelty effectiveness $\Gamma$:

$$\Gamma = \frac{d\mathbf{E}[\mathcal{R}|\mathcal{N}]}{d\mathcal{N}} = \beta_{\mathcal{N}} \quad (7)$$

The higher $\Gamma$ is, the greater overall payoff one sees for increasing novelty. Figure 10 shows our second result: a positive novelty bias for $\Gamma$ from small scale to about 300 speeches. Throughout this work, we use these measures at different scales $w$. Figure 9 contains transience v. novelty and resonance v. novelty density plots at several example scales.

*2.1. Presidential speech removal*

Our analysis is focused on innovation and generation and disposal of content in the NCA. Because the president functions as an enforcer of the agenda, his speeches are much more formulaic in content than others. He often maintains order and announces the transition from one speaker to the next, in addition to introducing the general topic of discussion. Some examples out of context:

```
<sp>
  <speaker>M. le Président</speaker>
  <p> le rappelle à l'ordre. </p>
</sp>

<sp>
  <speaker>M. le Président.</speaker>
  <p> Monsieur Pétion , je vous rappelle à l'ordre.</p>
</sp>

<sp>
  <speaker>M. le Président</speaker>
  <p> annonce à l'Assemblée qu'il a présenté
  différents décrets à la sanction du roi. </p>
 </sp>

<sp>
  <speaker>M. le Président.</speaker>
  <p> Il faut auparavant délibérer sur la motion d'inscrire sur le
  procés-verbal l'explication donnée par MM. l'abbé Grégoire et de
  Mirabeau. </p>
</sp>

<sp>
  <speaker>M. le Président.</speaker>
  <p> Un de MM. les secrétaires va faire l'appel nominal, pour que les
  ecclésiastiques fonctionnaires publics...</p>
</sp>

<sp>
  <speaker>M. le Président.</speaker>
  <p> Je vais consulter l'Assemblée pour savoir si elle entend fermer la
  discussion. </p>
  <p>(Une première épreuve a lieu ; elle est déclarée douteuse.) . </p>
</sp>
```

We can see the effect this constraint on the president's speech has by measuring role-reflexive novelty, transience, and resonance: when a center speech is classified as presidential, new-item committee, or in-debate committee (committee appendix) we use KLD measurements from only window speeches of the

same class. As an example, role-reflexive presidential innovation measures how divergent the president is from his own speech at a particular scale. As Figure 20 shows, the president is the least surprising compared to his own speech (novelty and transience), likely due to the constraints the role places on his conduct. Because of this formulaic nature, we remove presidential speeches from measurement windows when calculating novelty, transience, and resonance (Figure 8). All results are calculated this way except for those shown in Figure 20.

### *2.2. Novelty, transience, and resonance over time*

Daily means of novelty, transience, and resonance are shown for scales 36 and 153 in Figures 11 and 12. The raw values for these scales are shown for the last month of the NCA in Figure 13. Because the FRDA doesn't include markup for sub-day time stamps, we space speeches within a day evenly over the 24 hours. In this figure we can see the effect of increasing scale: visually apparent daily patterns for resonance at scale 36 average out to multi-day ones at scale 153. These periodicities in resonance can be seen directly in the Lomb-Scargle periodograms (see Refs. [21, 22]; Ref. [23] for application to behavioral data) for the final calendar year of the Assembly at differing scales (Figure 16). The daily pattern for scale 36 is evident in the power spike at $\sim$30 times a month. Scale 153 shows more power concentrated at lower frequencies, and at much higher scale 874 we see monthly trends come to the fore. Interestingly, the power spectra for the previous two calendar years are not as neatly defined (Figures 14 and 15, with direct year comparisons in Figure 17.)

## 3. Role behavior

Debate at the NCA's inception was chaotic, hampering progress towards the body's goals. Gradually, however, the Assembly developed official rules and tacit practices to regulate debate. In an early advance, the Assembly passed a generalized *règlement* in late July 1790 establishing simple majority from at least 200 delegates as sufficient conditions for passing decrees. The document also created the positions of president and six secretaries, usually two of whom recorded the minutes at any one time. Its rules governing debate were treated as guidelines, and the structure of debate continued to evolve organically until the Assembly's conclusion[14]. The committees embodied this evolutionary process. Each was created to handle a specific area of concern, typically crafting initial versions of decrees and presenting them to the Assembly. This pattern started before even the creation of the presidency, since the Rules Committee was given the responsibility to draft the aforementioned *réglement*[14].

These committees became indispensable workhorses for the emerging government:

> In many respects, the single most important organizational development was the emergence of the committee system...By 1790 the committees had become the workshops in which new laws and articles to the constitution were developed and initially debated. Most motions

> were systematically referred to committees before being considered in the full Assembly, so that their work came to set the rhythms of the constitutional process. To be sure, committee proposals were rarely accepted unchanged and without debate, particularly in the early months of the Assembly's existence[14].

The committees, however, became powerful entities themselves:

> As the deputies moved beyond debates on the guiding principles and general division of power within the constitution, and as they concentrated more on the technical details of implementation, it was evident that the committees alone had the expertise necessary for understanding the full ramifications of many laws. 'These committees,' wrote Dinochau, 'regulate the order of debate, classify questions, and maintain a continuity of principles, thus preventing an incoherence which might otherwise have menaced our decrees.'...Indeed, the committees became increasingly powerful not only within the National Assembly, but within the royal government as well. Whatever the deputies' early reticence to assume the powers of the 'executive,' the ministers were soon deferring to the Assembly on all manner of questions, refusing to take responsibility for decisions without the authority of the appropriate committees. Since 'executive authority was playing dead'—in Charles de Lameth's phrase—the committees emerged as veritable de facto ministries. Men like Roederer on the Tax Committee, Gregoire and Durand de Maillane on the Ecclesiastical Committee, or Merlin ('the Sorcerer') on the Feudal Committee undoubtedly knew more about their areas of concern and wielded more real power in the implementation of laws than any of the corresponding ministers[14].

The president enforced the agenda, while proxies for each committee presented their committees' proposed articles and decrees for debate. We split committee speech into two classes: new-item, presenting decrees before consumption, and in-debate, engaging in direct discussion with delegates. Details are in the Defining Committee Speech appendix.

Figure 18 shows monthly speech counts and proportions for each of the three roles as well as their complement, encompassing general legislative speech. As the NCA developed organically, committee speech took a greater portion of the proceedings, eventually equaling that of the president. Figure 19 shows some characteristics of these roles in waiting time distributions. All three roles exhibit long tails compared to general debate speech. This is likely a feature of their debate-managing functions: they either enforce what content is discussed at what time or provide the content to be processed, bookending periods of general proceedings. Interestingly, the president's tail is easily shorter than the committees' pre-1791. This may be due to the immaturity of the committees' function, leaving more organizational room for the president to be "hands-on" with greater regularity before the committees "set the rhythm" of debate as

quoted above. In 1791, the president's distribution seems to conform more to the committees'.

Although the president enforced the agenda, his powers were limited:

> In reality, the considerable potential powers of the president were substantially reduced by the short, two-week duration of his tenure. While several individuals held the post more than once' including Thouret who held it four times, and André and Bureaux de Pusy who held it three times each' no one after Bailly held it twice in succession. In general, moreover, the presidents were closely scrutinized by the Assembly in all their actions and were vigorously taken to task if they failed to follow the rules or seemed openly to favor one faction over another. They frequently felt compelled to consult the full Assembly whenever important controversies arose: on whether individual deputies should be allowed to speak out of order, for example. Nevertheless, the president remained the ceremonial center of the National Assembly and the chief representative of that body in relations with the king and his ministers. In most day-to-day affairs he exercised considerable control over the speaker's platform and played a central and often dominant role in establishing the subject and sequence of debate and in assuring the order and continuity which the early assemblies had so badly lacked. In practice, moreover, many of the individuals chosen were powerful personalities, skillful in speaking and in asserting leadership. [14]

Paradoxically, the assembly took the president to task when he "failed to follow the rules" (above), forcing the current holder of the powerful position into a tightly-bound set of behavior. This account illustrates the presidency as a highly constrained power, operating formulaically at the behest of the Assembly.

We see evidence of this in Figure 20, where we calculate mean novelty, transience, and resonance "reflexively" for each role. "Reflexive" means that novelty, transience, and resonance are calculated using only speeches that match the center speech's role. A presidential speech is compared to only other presidential speeches, etc. Past scale 10, the president is the most self-similar, even when compared to general speech, which is intuitively likely to be similar because of its serial nature in conversation. We take this as evidence for the president's formulaic nature, using a much more consistent vocabulary than general debate and other roles. We also see corroboration of other roles' function in this figure: As the provider of new material, instigating debate on new topics, new-item committee speech is the least self-similar. Given its more debate-centric nature, in-debate committee speech is more self-similar, but not as much as general speech.

## 4. Defining committee speech

The minutes of the NCA contain syntactic markers identifying whenever a committee representative speaks, taking the form of preambles to the actual

output of the speaker. Below is an example of the preamble “au nom du comité” identifying the individual as speaking “in the name of” the finance committee.

```
<sp>
 <speaker>M. Le Couteulx de Canteleu</speaker>
 <p>,au nom du comit\'{e} des finances, présente le projet de décret suivant,
 qui est adopté sans discussion : </p>
 <p>L'Assemblée nationale, sur le rapport de son comit\'{e} des finances,
 décrè}te ce qui suit : </p>
 <p>Art. 1<hi rend="superscript">er</hi>.</p>
 <p> Le directeur général du Trésor public est autorisé d'établir, sous
 sa direction et sa surveillance, un bureau de correspondance générale
 avec les receveurs de district, formé en quatre sections, entre
 lesquelles seront partagés les quatre-vingt trois départements, avec un
 directeur et deux chefs de bureauà chaque section, et autant de commis
 qu'il sera nécessaire. Les comptes de chacun des receveurs de district
 y seront tenus en partie double, pour s'assurer dè} la recette effective
 et des sommesà disposerà terme fixe, pour les besoins du Trésor
 public. </p>
 <p>Art. 2.</p>
 ...
</sp>
```

We find several preambles in the corpus, contained in Table 5 with our labels for each in analysis, the general form of the preamble, and the regular expressions used in the search. Once cleaned of punctuation, these preambles occur as the first words in a speech. Regular expressions match only at the beginning of cleaned speech text. Figure 21 shows the gradually increasing proportion of these markers over time.

To learn the function of each of these markers in the debate stream, we obtain random samples of each from before and after January 1, 1791. We rate each speech on three categories: i) whether the speech is, in fact, spoken by a committee member, ii) whether the speech contains a new item of discussion in the proceedings, and iii) whether it presents official output. For category (i), we examine context in the AP to see whether the speaker associated with the marker is explicitly identified as a committee proxy. To rate category (ii), we examine context again, looking through previous speeches to see whether the speech in question broached a new item or fell in the period of discussion after an item's introduction. “New items” quite often include starting proceedings as an order of the day or an agenda item. We also see blocks of new items (decrees, proposals, etc.) introduced in succession by the same committee, where each is a separate and specific issue even if collected under a general theme. Each of these is considered a new item in our analysis. We define official output in category (iii) as decrees or articles prepared by the committee and read aloud or presented as an official creation of the Assembly. Reports made in the vernacular are not considered official.

Table 6 contains our ratings for each sample. Rating labels IsCommittee, NewItem, and OfficialOutput, represent categories (i), (ii), and (iii). “nom comité” and “rapporteur comité” markers are much more likely to mark the presentation of new items to the Assembly rather than engage in debate. Qualitatively, we notice a rough pattern of these more formal preambles introducing delegates presenting new items in the agenda. If a committee member engages

| Label | General form |
|---|---|
| nom comité | au nom du comité |
| rapporteur comité | rapporteur du comité |
| membre comité | membre du comité |
| rapporteur | rapporteur (without "du comité" following) |
| **Label** | **General regular expression** |
| nom comité | (au—ai—an—ûu—aïi—cm—du—m—nu—qu) nom (du—des?—dû—au—dif—jtu—èu—la)(  ces)?(  v)?( deux)?( trois)? (comité—comitis—cemité—oomité—comite) |
| rapporteur comité | rapporteur (du—des?—dtt—dû) comité |
| membre comité | membre du (c—b—è—e)omité |
| rapporteur | rapporteur(?! (du—des?—dtt—dû) comité) |
| **Label** | **Outlier regular expressions** |
| nom comité | 1. de coulantes au nom du |
| | 2. aainéau nom du comité |
| | 3. cidevan t de vieuzac au nom fiu comité |
| | 4. présenteau nom du comité |
| | 5. de saintlô au nom des comités |
| | 6. de bigarre au nom du comité des finances |
| | 7. de coùtances au nom du comité |
| | 8. de coûtantes au nom dy comité |
| | 9. nom du comité central |
| | 10. vaainé au nom des comités |
| | 11. au nom ducomité d agriculture |
| rapporteur comité | 1. comme rapporteur du comité |
| membre comité | 1. de baigorre membre du comité |
| | 2. membre et organe du comité |
| | 3. piempre du comité |

Table 5: Labels, general forms, and regular expressions for each committee speech preamble marker. Regular expressions search for a variety of OCR and grammatical variations including plural usage, articles, etc. Data matched are the raw speeches cleaned of punctuation, set to lower case, having single space characters between words. Outlier expressions are those found in the manual search and sample-taking process.

in a debate after the item's introduction, then less formal appellations are used: "rapporteur" or "membre comité." This pattern is not always the case: as one can see in the NewItem column of Table 6, "rapporteur"-marked delegates do sometimes present new items, for instance when the president announces their committee credentials beforehand. As a last comment on these marker ratings, "rapporteur" is not reliably rated positively for category (i), IsCommittee. This is due to lack of *explicitly* stated association to a particular committee in context. The content presented was often implicitly committee-produced or very similar to committee output.

| Label | IsCommittee | OfficialOutput | NewItem | Sample Size |
|---|---|---|---|---|
| Before 1791-01-01 | | | | |
| rapporteur | 6 | 7 | 4 | 10 |
| membre comité | 13 | 6 | 9 | 13 |
| rapporteur comité | 10 | 7 | 10 | 10 |
| nom comité | 10 | 9 | 10 | 10 |
| After 1791-01-01 | | | | |
| rapporteur | 6 | 6 | 2 | 10 |
| membre comité | 10 | 5 | 5 | 10 |
| rapporteur comité | 10 | 9 | 8 | 10 |
| nom comité | 10 | 8 | 8 | 10 |

Table 6: Aggregated ratings for committee marker samples before and after 1791-01-01. "nom comité" and "rapporteur comité" markers are much more likely to mark the presentation new items to the Assembly rather than engage in debate. An explicit connection to a committee was not always found for the "rapporteur" marker, producing lower IsCommittee counts, but the content reported qualitatively matched typical committee output.

Based on the ratings, we group markers into two classes, in-debate ("rapporteur" and "membre comité") and new-item ("nom comité" and "rapporteur comité"). Table 7 contains the speech count breakdown of each class and marker, and Figure 22 shows their monthly proportion of all speeches over time.

### *4.1. Committee speech and information processing*

Figure 23 shows the speech-level relationship between resonance and novelty in scatter plots for several scales with speeches split into new-item, in-debate, and non-committee speech. Each scale shows speeches before and after 1791-10-31, the epoch dividing point found for the scale range most sensitive to new-item committee effect on $\Gamma$ (see diachronic modeling appendix). One can see the development of a tail for high novelty as scale increases above 7, and only in the second epoch. We mark each plot with a threshold of convenience, $z(\mathcal{N}) = 3$, for comparison between epochs. In Figures 23 and Figure 24, new-item speech seems to dominate the tail. In Figure 24, we see that the tail also contains in-debate and non-committee speech. We account for the appearance of non-committee speech in the tail in the next paragraph.

| Label | Pre-1791-01-01 | Post-1791-01-01 | NCA Total |
|---|---|---|---|
| in-debate committee speech class | | | |
| membre comité | 235 | 14 | 249 |
| rapporteur | 819 | 3,243 | 4,062 |
| new-item committee speech class | | | |
| nom comité | 243 | 1,205 | 1,448 |
| rapporteur comité | 242 | 38 | 280 |
| non-committee | 20,493 | 18,421 | 38,914 |
| Grand total | | | 44,953 |

Table 7: Counts and assignment of committee speech preamble labels to in-debate and new-item speech classes, before and after 1791-01-01.

To investigate the composition of tail speeches, we obtain the intersection of speeches above $z(\mathcal{N}) = 3$ for each class over scales 17, 36, and 153. Accounting is shown in Table 8. We sample the intersection and rate the resulting speeches for new-item status and official output as before. We add rating categories for a) the number of speeches contained within the OCR-defined speech as presented in the FRDA XML and b) whether the sampled speech contains committee speech. There were only ever one or two speeches contained within a sampled speech, so we use labels SpeechCount1 and SpeechCount2 to represent the number of sampled XML speeches containing one and two "real" speeches for category (a). We label category (b) with ContainsCommittee (similar to category (i), IsCommittee, but for multiple, erroneously combined, "real" speeches).

Table 9 contains the rating results. The non-committee tail sample always has committee speech within it, sometimes as a second sub-speech due to OCR error, presenting new items to the Assembly. Therefore, tail speeches in the non-committee class seem to be misdiagnosed, and should be considered part of the new-item class. Because of their relatively low prevalence in the tail compared to classified new-item speech, and because of a lack of easily-defined machine-readable markers for these misdiagnosed speeches, we leave the committee speech classifications as-is.

## 5. Synchronic modeling of role behavior

According to historian Timothy Tackett, "the single most important source of prominence and impact within the Assembly was an individual's success at the speaker's rostrum...a successful and compelling manipulation of the spoken language became one of the most important–though certainly not the only–sources of power within the Assembly."[14] As time progressed, a small fraction of all delegates came to dominate discussion. "Examining the roster of the top forty [orators], one is impressed by the presence of the lesser known deputies

| Scale | Speech class count | | |
|---|---|---|---|
| | Non-committee | In-debate | New-item |
| 17 | 61 | 35 | 143 |
| 36 | 48 | 40 | 150 |
| 153 | 49 | 45 | 146 |
| Intersection | 35 | 23 | 124 |

Table 8: Counts of committee speech classes above tail threshold for scales 17, 36, and 153, with size of the speech class intersection across scale. After analysis, non-committee tail speeches ($z(\mathcal{N}) > 3$) tend to be misclassified by the regex search procedure and should be considered new-item (Table 9).

| Rating | Speech class count | |
|---|---|---|
| | Non-committee | New-item |
| SpeechCount1 | 4 | 9 |
| SpeechCount2 | 6 | 1 |
| ContainsCommittee | 10 | 10 |
| OfficialOutput | 10 | 10 |
| NewItem | 10 | 10 |
| Sample Size | 10 | 10 |

Table 9: Aggregated ratings for samples of each speech class in the tail, above $z(\mathcal{N}) = 3$. SpeechCount1 and SpeechCount2 are the number of sampled speeches that actually contain one or two "real" speeches within them; those with two are misread during OCR. The non-committee tail sample always has committee speech within it, sometimes as a second sub-speech due to OCR error, presenting new items to the Assembly. Tail speeches in the non-committee class seem to be misdiagnosed, and should be considered part of the new-item class.

Camus, Andre, Demeunier, Regnaud, Bouche, Gaultier de Biauzat, and Goupil, interspersed among such high-profile personalities as Mirabeau, Barnave, Malouet, and Maury. Though the index can tell us nothing of the quality and impact of such oratory, it would suggest nevertheless that oratorical leadership in the Assembly went well beyond the 'great speakers' who figure most prominently in the standard accounts of the Revolution."[14] Although $\mathcal{R} \propto \mathcal{N}$ at the speech level, the various characteristics of an orator–his demeanor, social standing, etc.–can break this overall trend. An unskilled, risk-prone delegate may "succeed" only rarely, accruing high mean novelty and low mean resonance scores.

In addition, an organization constrains an orator's behavior using an agenda, a code of conduct, etc. The organization extends its powers by creating official positions tasked with a particular functions. An example is the president of the Assembly, created as a point of contact for the King and an enforcer of the daily agenda[14]. Delegates rotated frequently through this position, taking

on its responsibilities as designated by the Assembly. The presidency then represents an organizationally imposed entity at the individual level, operating with a contiguous code of conduct no matter who was filling the position.

The Assembly created another specialized entity: the committee. Committees developed content outside of the debate process, presenting official documents for review on the debate floor in accordance with the agenda. The recorders of the NCA used a system of lexical markers to identify when a committee member was speaking. We catalog these and organize them into two semantic classes: "new-item" and "in-debate" committee speech (see the appendix on defining committee speech). New-item speeches introduce official content to the Assembly floor, typically articles and draft decrees to be reviewed by the legislative body. As the harbingers of debate on official output of the NCA, these speeches mark shifts between periods of governmental attention on specific items. In-debate committee speeches occur when a committee member or reporter engages with other delegates in the midst of debate on some item. In the minutes, one will often see an "order of the day" or agenda item announced by the president, directly followed by a new-item committee speech presenting an official document before a period of debate. Sometimes this debate is punctuated by "live" editing of the document by committee members, each marked by in-debate speech cues. Rotating committee members, delivering either new-item or in-debate speech, take on the responsibilities of the post. In this way, committee proxies are another organizationally imposed entity shaping discourse.

To understand synchronic informational roles in the system, we calculate mean z-scored novelty and resonance at scales from 1 to 5,000 for the top forty orators, the presidency, and both committee classes. Table 10 contains these quantities for scale 36. [table description]

In Figure 25, left plot, we see the outstanding novelty associated with new-item speech, and at larger scale, in-debate speech. As gatherers of new information, the committees act as information injectors through their proxies in debate. In addition, we see that many individuals' profiles in novelty are readily separable and stable over large scale ranges. This is not the case for resonance (Figure 25, right plot), where substantially fewer individuals are measurably and reliably resonant or anti-resonant.

Combining an entity's innovation and resonance outlines its informational role in the Assembly. The new-item combination of high novelty and high resonance embodies the positive relationship shown at the speech level. In contrast, the presidency shows greater novelty than normal (dipping lower at high scale), but lesser resonance. As an enforcer of debate, the president must break from preceding topics to further the agenda. However, he does not introduce new information to be immediately processed as does the new-item committee proxy.

### *5.1. Consistency of measurements over multiple timescales*

In the main paper, we report results at the individual/role level for $w$ equal to 36. How consistent are these results at longer, or shorter timescales? Fig. 27

| Name | $z(\mathcal{N})$ | $z(\mathcal{R})$ | $\Delta z(\mathcal{R})$ | Type |
|---|---|---|---|---|
| High novelty, high resonance | | | | |
| Jérôme Pétion de Villeneuve | 0.10 | 0.28*** | +0.25*** | 3g |
| Maximilien Robespierre | 0.11** | 0.18*** | +0.14** | 3g |
| Jean-Denis Lanjuinais | 0.06 | 0.16*** | +0.15*** | 3g |
| Alexandre Lameth | 0.17** | 0.14* | +0.09 | 2g |
| Charles Antoine Chasset | 0.31*** | 0.13* | +0.04 | 3g |
| new_item | 1.31*** | 0.12*** | -0.27*** | — |
| Adrien Duport | 0.07 | 0.05 | +0.03 | 2g |
| Philippe-Antoine Merlin (de Douai) | 0.27*** | 0.05 | -0.03 | 3g |
| Jean-Nicolas Démeunier (Desmeunier) | 0.01 | 0.03 | +0.03 | 3- |
| Pierre-Franҫis Gossin | 0.65*** | 0.03 | -0.17** | 3g |
| Michel Louis Etienne Regnaud | 0.00 | 0.02 | +0.02 | 3g |
| in_debate | 0.29*** | 0.02 | -0.07*** | — |
| Jean-Louis Emmery | 0.07 | 0.02 | 0.00 | 3g |
| Jacques Franҫis Menou | 0.40*** | 0.02 | -0.10 | 2g |
| Isaac René Le Chapelier | 0.06 | 0.01 | -0.01 | 3g |
| High novelty, low resonance | | | | |
| Jacques Guillaume Thouret | 0.16*** | 0.00 | -0.05 | 3g |
| Jean Baptiste Chabroud | 0.09 | -0.02 | -0.04 | 3g |
| Jacques Joseph Defermon de Chapelières | 0.35*** | -0.03 | -0.13** | 3- |
| Honoré Gabriel Riqueti Mirabeau | 0.03 | -0.04 | -0.04 | 3g |
| Franҫis Denis Tronchet | 0.24*** | -0.04 | -0.11 | 3g |
| Armand-Gaston Camus | 0.29*** | -0.04 | -0.13*** | 3g |
| Emmanuel[...] Fréteau de Saint Just | 0.01 | -0.05 | -0.06 | 2g |
| president | 0.02 | -0.07*** | -0.08*** | — |
| Théodore Vernier | 0.55*** | -0.14** | -0.31*** | 3g |
| Low novelty, high resonance | | | | |
| Guillaume Franҫis Charles Goupil-Préfelne | -0.21*** | 0.13** | +0.20*** | 3g |
| Jean-Franҫis Reubell | -0.18*** | 0.11* | +0.16*** | 3g |
| Louis Simon Martineau | -0.05 | 0.08* | +0.10** | 3g |
| Jacques Antoine Marie Cazalès, de | -0.44*** | 0.08* | +0.21*** | 2d |
| Pierre Victor Malouet | -0.27*** | 0.08* | +0.16*** | 3d |
| Louis Marie Estourmel, d' | -0.26*** | 0.07 | +0.15* | 2d |
| Jean-Sifrein Maury | -0.46*** | 0.07 | +0.20*** | 1d |
| Pierre-Louis Prieur [dit Prieur de la Marne] | -0.27*** | 0.05 | +0.13*** | 3g |
| Jean-Franҫis Gaultier de Biauzat | -0.13** | 0.03 | +0.06 | 3g |
| Antoine Balthazar Joseph André, d' | -0.03 | 0.02 | +0.03 | 2g |
| Low novelty, low resonance | | | | |
| Dominique Garat | -0.13** | 0.00 | +0.04 | 3g |
| Antoine Charles Gabriel Folleville | -0.44*** | -0.01 | +0.12** | 2d |
| Louis-Michel Le Peletier de Saint-Fargeau | -0.20*** | -0.01 | +0.05 | 2g |
| Franҫis Dominique de Reynaud Montlosier | -0.61*** | -0.02 | +0.17** | 2d |
| Pierre-Louis Roederer | -0.10* | -0.03 | 0.00 | 3g |
| Louis Foucauld de Lardimalie | -0.53*** | -0.05 | +0.11* | 2d |
| Charles Malo F Lameth | -0.15*** | -0.06 | -0.02 | 2g |
| Pierre Franҫis Bouche | -0.09** | -0.10* | -0.07 | 3g |
| Antoine Barnave | -0.04 | -0.12* | -0.11* | 3g |

Table 10: Means/t-test entity categorization table, now including non-significant detections; $w$ equal to 36 (as shown in main text).

plots the Pearson correlation with the reported results for novelty, resonance, and $\Delta R$ (resonance over/under the group-level prediction) as a function of $w$.

Novelty is very consistent on timescales from minutes (speech-to-speech) to months ($w$ equal to 5000, the limit of our data); transience (not shown) follows a very similar curve. Interestingly, $\Delta R$ is more consistent than resonance itself. Tables 11 and 12 show the results for the two extreme timescales ($w$=1, or "speech-to-speech", and $w$ equal to 5000, equivalent to timescales of months).

## 6. Diachronic modeling of role behavior

### *6.1. Single epoch model*

We start with a simple linear model,

$$\mathbf{E}[\mathcal{R}|\mathcal{N}] = \beta_{int} + \beta_{\mathcal{N}}\mathcal{N} + \sigma. \tag{8}$$

extending it to include time effects:

$$\mathbf{E}[\mathcal{R}|\mathcal{N}, t] = \beta_{int} + \beta_t t + (\beta_{\mathcal{N}} + \beta_{\mathcal{N}t} t)\mathcal{N} + \sigma \tag{9}$$

Novelty effectiveness then becomes a function of time:

$$\Gamma(t) = \frac{\partial \mathbf{E}[\mathcal{R}|\mathcal{N}, t]}{\partial \mathcal{N}} = \beta_{\mathcal{N}} + \beta_{\mathcal{N}t} t \tag{10}$$

Fitting Eq. 9 using OLS regression on z-scored $\mathcal{R}$ and $\mathcal{N}$ over a selection of increasing scales produces the trend lines in Figure 28. Parameter estimates with confidence intervals are shown in Figure 29. The effectiveness of novelty decreases with time over all but the highest scales (Figure 29). According to this single epoch model, discourse in the NCA becomes inexorably more intolerant of novelty.

Modeling $\Gamma$ specifically for committee speech tells a more complex story. Monthly $\Gamma$s, fit using Eq. 6 and split into new-item committee vs. all other speech, show a divergence in behavior: new-item $\Gamma$ drops during the final year of the NCA (Figure 30). The single epoch model cannot account for this change.

### *6.2. Two-epoch models*

Historian Timothy Tackett describes a divergence of roles taken on by delegates in the Assembly. While bombastic orators won the battle for influence on the debate floor, those with ambitious but unassuming souls entered committees and collectively gained power[14]. As time went on, committees gained more and more influence, becoming "de facto ministries," independent of the blessing of debaters in the general NCA[14]. To explore the role played by new-item committee proxies, we develop a two-epoch model of the NCA. The first epoch

| Name | $z(\mathcal{N})$ | $z(\mathcal{R})$ | $\Delta z(\mathcal{R})$ | Type |
|---|---|---|---|---|
| | | High novelty, high resonance | | |
| new_item | 1.23*** | 0.32*** | -0.39*** | — |
| Pierre-Françis Gossin | 0.37*** | 0.08 | -0.13* | 3g |
| Jacques Guillaume Thouret | 0.06 | 0.07 | +0.04 | 3g |
| Jacques Joseph Defermon de Chapelières | 0.16** | 0.06 | -0.04 | 3- |
| Charles Antoine Chasset | 0.13 | 0.05 | -0.03 | 3g |
| Jacques Françis Menou | 0.19* | 0.04 | -0.07 | 2g |
| Jérôme Pétion de Villeneuve | 0.03 | 0.04 | +0.02 | 3g |
| Maximilien Robespierre | 0.01 | 0.02 | +0.01 | 3g |
| in_debate | 0.02 | 0.01 | +0.00 | — |
| | | High novelty, low resonance | | |
| Armand-Gaston Camus | 0.23*** | -0.01 | -0.14*** | 3g |
| Philippe-Antoine Merlin (de Douai) | 0.16** | -0.01 | -0.10* | 3g |
| Jean Baptiste Chabroud | 0.02 | -0.02 | -0.03 | 3g |
| Honoré Gabriel Riqueti Mirabeau | 0.02 | -0.03 | -0.04 | 3g |
| Emmanuel[...] Fréteau de Saint Just | 0.03 | -0.06 | -0.08* | 2g |
| Michel Louis Etienne Regnaud | 0.02 | -0.09* | -0.11** | 3g |
| president | 0.14*** | -0.10*** | -0.18*** | — |
| Théodore Vernier | 0.46*** | -0.12 | -0.39*** | 3g |
| | | Low novelty, high resonance | | |
| Guillaume Françis Charles Goupil-Préfelne | -0.02 | 0.15** | +0.16*** | 3g |
| Jacques Antoine Marie Cazalès, de | -0.14*** | 0.07 | +0.15*** | 2d |
| Louis-Michel Le Peletier de Saint-Fargeau | -0.18*** | 0.07 | +0.18*** | 2g |
| Louis Marie Estourmel, d' | -0.14* | 0.06 | +0.15** | 2d |
| Adrien Duport | -0.01 | 0.06 | +0.06 | 2g |
| Antoine Charles Gabriel Folleville | -0.13* | 0.06 | +0.13*** | 2d |
| Louis Simon Martineau | -0.02 | 0.04 | +0.05 | 3g |
| Jean-Françis Reubell | -0.09 | 0.02 | +0.07 | 3g |
| Isaac René Le Chapelier | -0.02 | 0.02 | +0.03 | 3g |
| Dominique Garat | -0.15** | 0.01 | +0.10* | 3g |
| Louis Foucauld de Lardimalie | -0.24*** | 0.01 | +0.14*** | 2d |
| Pierre Victor Malouet | -0.17*** | 0.00 | +0.10*** | 3d |
| | | Low novelty, low resonance | | |
| Jean-Denis Lanjuinais | -0.03 | 0.00 | +0.01 | 3g |
| Jean-Sifrein Maury | -0.26*** | -0.02 | +0.14*** | 1d |
| Antoine Barnave | -0.03 | -0.03 | -0.01 | 3g |
| Charles Malo F Lameth | -0.14** | -0.03 | +0.05 | 2g |
| Pierre Françis Bouche | -0.03 | -0.03 | -0.01 | 3g |
| Alexandre Lameth | -0.04 | -0.04 | -0.02 | 2g |
| Antoine Balthazar Joseph André, d' | -0.05 | -0.04 | -0.01 | 2g |
| Jean-Françis Gaultier de Biauzat | -0.14** | -0.04 | +0.04 | 3g |
| Jean-Nicolas Démeunier (Desmeunier) | -0.07* | -0.04 | -0.01 | 3- |
| Pierre-Louis Prieur [dit Prieur de la Marne] | -0.25*** | -0.05 | +0.10*** | 3g |
| Françis Dominique de Reynaud Montlosier | -0.45*** | -0.06 | +0.20*** | 2d |
| Françis Denis Tronchet | -0.08 | -0.06 | -0.01 | 3g |
| Pierre-Louis Roederer | -0.13** | -0.09 | -0.02 | 3g |
| Jean-Louis Emmery | -0.07 | -0.12 | -0.08 | 3g |

Table 11: Means/t-test entity categorization table, now including non-significant detections. $w$=1; speech-to-speech microscale.

| Name | $z(\mathcal{N})$ | $z(\mathcal{R})$ | $\Delta z(\mathcal{R})$ | Type |
|---|---|---|---|---|
| | | High novelty, high resonance | | |
| Jérôme Pétion de Villeneuve | 0.27*** | 0.32*** | +0.30*** | 3g |
| Antoine Barnave | 0.25*** | 0.29*** | +0.28*** | 3g |
| Isaac René Le Chapelier | 0.13*** | 0.23*** | +0.22*** | 3g |
| Maximilien Robespierre | 0.23*** | 0.19*** | +0.18** | 3g |
| Adrien Duport | 0.30*** | 0.19** | +0.17** | 2g |
| Pierre-Louis Roederer | 0.08 | 0.17*** | +0.17*** | 3g |
| Jacques Franҫis Menou | 0.46*** | 0.17** | +0.14* | 2g |
| Charles Antoine Chasset | 0.36*** | 0.13* | +0.11 | 3g |
| Honoré Gabriel Riqueti Mirabeau | 0.07 | 0.12** | +0.12** | 3g |
| Pierre-Franҫis Gossin | 0.60*** | 0.10 | +0.06 | 3g |
| Jacques Joseph Defermon de Chapelières | 0.41*** | 0.09 | +0.06 | 3- |
| Armand-Gaston Camus | 0.28*** | 0.08* | +0.06 | 3g |
| Jean-Denis Lanjuinais | 0.01 | 0.07 | +0.07 | 3g |
| Jacques Guillaume Thouret | 0.33*** | 0.07 | +0.05 | 3g |
| in_debate | 0.44*** | 0.06** | +0.03 | — |
| new_item | 1.18*** | 0.03 | -0.03 | — |
| | | High novelty, low resonance | | |
| Franҫis Denis Tronchet | 0.56*** | -0.06 | -0.09 | 3g |
| Théodore Vernier | 0.50*** | -0.09 | -0.12* | 3g |
| Jean Baptiste Chabroud | 0.10* | -0.10 | -0.11 | 3g |
| Philippe-Antoine Merlin (de Douai) | 0.29*** | -0.11* | -0.13** | 3g |
| Alexandre Lameth | 0.28*** | -0.12* | -0.13* | 2g |
| Jean-Louis Emmery | 0.02 | -0.18* | -0.18* | 3g |
| Louis-Michel Le Peletier de Saint-Fargeau | 0.33*** | -0.20* | -0.22** | 2g |
| Jean-Nicolas Démeunier (Desmeunier) | 0.17*** | -0.20*** | -0.21*** | 3- |
| | | Low novelty, high resonance | | |
| Jean-Sifrein Maury | -0.28*** | 0.39*** | +0.41*** | 1d |
| Jacques Antoine Marie Cazalès, de | -0.24*** | 0.28*** | +0.29*** | 2d |
| Antoine Charles Gabriel Folleville | -0.44*** | 0.27*** | +0.30*** | 2d |
| Michel Louis Etienne Regnaud | -0.03 | 0.17*** | +0.17*** | 3g |
| Guillaume Franҫis Charles Goupil-Préfelne | -0.24*** | 0.16** | +0.18** | 3g |
| Louis Simon Martineau | -0.06 | 0.16*** | +0.16*** | 3g |
| Franҫis Dominique de Reynaud Montlosier | -0.59*** | 0.11 | +0.15* | 2d |
| Charles Malo F Lameth | -0.07 | 0.10 | +0.10 | 2g |
| Louis Foucauld de Lardimalie | -0.47*** | 0.08 | +0.10 | 2d |
| Pierre Franҫis Bouche | -0.22*** | 0.05 | +0.06 | 3g |
| | | Low novelty, low resonance | | |
| Louis Marie Estourmel, d' | -0.32*** | 0.00 | +0.02 | 2d |
| Pierre Victor Malouet | -0.25*** | -0.01 | +0.01 | 3d |
| Jean-Franҫis Reubell | -0.27*** | -0.07 | -0.05 | 3g |
| Dominique Garat | -0.05 | -0.10 | -0.09 | 3g |
| Pierre-Louis Prieur [dit Prieur de la Marne] | -0.34*** | -0.10 | -0.08 | 3g |
| president | -0.08*** | -0.11*** | -0.11*** | — |
| Antoine Balthazar Joseph André, d' | -0.03 | -0.13** | -0.13** | 2g |
| Jean-Franҫis Gaultier de Biauzat | -0.22*** | -0.19** | -0.17** | 3g |
| Emmanuel[...] Fréteau de Saint Just | -0.04 | -0.26*** | -0.26*** | 2g |

Table 12: Means/t-test entity categorization table, now including non-significant detections. $w$=5000; largest timescales available in data.

considers reception of committee and non-committee speeches to be the same so uses the simplest linear model in Eq. 6:

$$\mathbf{E}[\mathcal{R}|\mathcal{N},\mathcal{C}] = \beta_{int} + \beta_{\mathcal{N}}\mathcal{N} + \sigma,$$

The second treats the two speech types differently by introducing categorical variable $C_n$ for new-item committee speech:

$$\begin{aligned}\mathbf{E}[\mathcal{R}|\mathcal{N},\mathcal{C}] = &\beta_{int} + \beta_{\mathcal{N}}\mathcal{N} + \beta_{\mathcal{C}_n}\mathcal{C}_n + \\ &\beta_{\mathcal{N}\mathcal{C}_n}\mathcal{N}\mathcal{C}_n + \sigma,\end{aligned} \tag{11}$$

We fit the overall model by searching for the maximum-likelihood partition of two epochs in monthly units, fitting each epoch to its respective linear sub-model separately. Parameter estimates and $R^2$ for this new-item, two-epoch model are shown in Figures 33 and 34. Resultant trend lines are added for new-item committee speech in Resonance v. Novelty scatter plots (Figure 32, second epoch). We constrain epoch length to be at least 4 months. As can be seen in Figure 31, the two-epoch model captures the committees' divergent Γ behavior. Figure 32 effectively illustrates this divergence in scatter plots of resonance and novelty for both epochs. Before 1790-10-31, new items presented by committees are treated similarly to other speech. Afterwards, we see new-item committee speech form an "efficient tail" – so named because of its comparatively low Γ (slopes of the trend lines shown in Figure 32). Consider two scenarios for a new item introduced to the speech stream, both with high novelty due to the inherent newness being presented. In the first, the floor takes up the new item and debates for a time. In the second scenario, the floor contributes little to no thoughts on the matter. In the latter scene, the transience of the speech is much higher than in the former, reducing resonance. Enough occurrences of the second scenario would drag the slope (Γ) of the resonance-novelty relationship down. This is what seems to happen in the second epoch for new items presented by committees. We discuss evidence for this no-debate hypothesis in the appendix on committee speech characterization.

As mentioned in the committee identification appendix, we find another class of "in-debate" committee speech. These speeches typically occur when committee members comment in the midst of debate on some item. We notice a pattern of item introduction by a committee member (a new-item committee speech), followed by general debate punctuated by committee member clarifications. Sometimes, these punctuations are actually "live" edits of official decrees presented by a committee member as the debate rolls forward. We can add another categorical speech class variable, $\mathcal{C}_d$ for in-debate, to the second epoch model:

$$\begin{aligned}\mathbf{E}[\mathcal{R}|\mathcal{N},\mathcal{C}_n,\mathcal{C}_d] = &\beta_{int} + \beta_{\mathcal{N}}\mathcal{N} + \beta_{\mathcal{C}_n}\mathcal{C}_n + \beta_{\mathcal{C}_d}\mathcal{C}_d + \\ &\beta_{\mathcal{N}\mathcal{C}_n}\mathcal{N}\mathcal{C}_n + \beta_{\mathcal{N}\mathcal{C}_d}\mathcal{N}\mathcal{C}_d + \sigma,\end{aligned} \tag{12}$$

$\Gamma$ then becomes

$$\Gamma(\mathcal{C}_n, \mathcal{C}_d) = \frac{\partial \mathbf{E}[\mathcal{R}|\mathcal{N}, \mathcal{C}_n, \mathcal{C}_d]}{\partial \mathcal{N}} = \beta_{\mathcal{N}} + \beta_{\mathcal{N}\mathcal{C}_n}\mathcal{C}_n + \beta_{\mathcal{N}\mathcal{C}_d}\mathcal{C}_d,$$

where setting $\mathcal{C}_n$ or $\mathcal{C}_d$ to 0 or 1 produces $\Gamma$ profiles for each of non-committee ($\Gamma_0$), new-item committee ($\Gamma_n$), and in-debate committee ($\Gamma_d$) speech classes:

$$\Gamma_0 = \Gamma(\mathcal{C}_n = 0, \mathcal{C}_d = 0) = \beta_{\mathcal{N}} \tag{13}$$
$$\Gamma_n = \Gamma(\mathcal{C}_n = 1, \mathcal{C}_d = 0) = \beta_{\mathcal{N}} + \beta_{\mathcal{N}\mathcal{C}_n} \tag{14}$$
$$\Gamma_d = \Gamma(\mathcal{C}_n = 0, \mathcal{C}_d = 1) = \beta_{\mathcal{N}} + \beta_{\mathcal{N}\mathcal{C}_d} \tag{15}$$

The effects committee speech classes have on $\Gamma$ are embodied in $\beta_{\mathcal{N}\mathcal{C}_n}$ and $\beta_{\mathcal{N}\mathcal{C}_d}$, measured relative to the non-committee baseline $\Gamma_0 = \beta_{\mathcal{N}}$. Each represents the effect of playing a particular role as a committee proxy. New-item committee speeches inject information into discourse, while those in-debate interact directly with the Assembly body during deliberation.

As before, we model each of the two epochs separately, using OLS regression and this model for each epoch and finding the best month partition date by maximum likelihood for the overall model. Estimated parameters for this all-committee, two-epoch model are shown in Figure 35; $R^2$ over scale is shown in Figure 37. The all-committee model is preferred by AIC over the single-epoch model for all scales 50. Figure 36 shows the committee $\Gamma$ parameters in context of resonance v. novelty scatter plots. The epoch-dividing change-points chosen over a range of scales cluster at the end of 1790 (Figure 38).

Committee members retain their power when in debate, shepherding conversation in both epochs. As discussed before, committee proxies delivering new items to the debate floor see a drop in $\Gamma$ in the second epoch.

*6.3. Explaining the time dependence in the single-epoch model*

We investigate the link between the single epoch model's temporal decrease in $\Gamma$ and the new-item committee speech, removing said speech before fitting another single-epoch model via Eq. 9. Comparisons of fit parameters and $R^2$ for the two models are shown in Figure 40. Figure 39 shows a general increase in $\partial\Gamma/\partial t$ for sampled scales after removal (compare to Figure 28). Notably, at scale 27 $\partial\Gamma/\partial t$ is no longer distinguishable from 0. Since the new-item drop in $\Gamma$ occurs only in the last year of the NCA, it manifests in a linearly decreasing $\Gamma$ over time in the single-epoch model. Figure 41 shows a comparison of $\partial\Gamma/\partial t$ over scale, with and without new-item speeches. Removing these speeches drives up the time slope across scale, most notably to 0 in the $\sim$20-60 speech scale range. This is exactly the range showing lowest values in new-item $\Gamma$. Without the shift in reception of new item speeches, the general $\Gamma$ for the NCA is constant over time at this scale range.

*6.4. Two-epoch model with fixed intercept*

The previous models show how returns to resonance $\Gamma$ evolve for each committee *internally.* To place each committee's resonance-novelty relationship in the context of the overall system, we fit another 2-epoch model where the intercepts of each role are fixed:

$$\mathbf{E}[\mathcal{R}|\mathcal{N}, \mathcal{C}_n, \mathcal{C}_d] = \beta_{int} + \Gamma_n \mathcal{N}\mathcal{C}_n + \Gamma_d \mathcal{N}\mathcal{C}_d + \sigma, \tag{16}$$

This is the model presented in the main paper. It retains the interaction terms and baseline intercept from Eq. 12, re-branding $\beta_{\mathcal{N}\mathcal{C}_n}$ as $\Gamma_n$ and $\beta_{\mathcal{N}\mathcal{C}_d}$ as $\Gamma_d$. This model allows us to compare each committee's resonance return to the other based on relative positions of each point cloud in the resonance-novelty plane. As in earlier results, new-item $\Gamma$ drops in the second epoch, which begins at the end of 1790 (Figures 43 and 45). Figure 43 is presented in the main paper. Modeling results are presented in Figures 42 and 44.

*6.5. Including all roles in the two-epoch model*

Figures 46 to 49 show the effect of adding a presidential categorical variable to the all-committee model, creating an all-role model. Although the latter model is preferred by AIC (Figure 50), the presidential addition does not change the results from the former model.

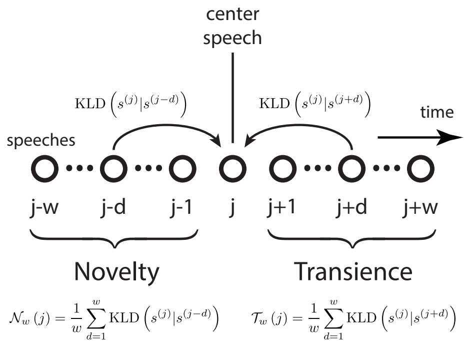


Figure 8: Diagram of novelty and transience. Each speech is represented by an LDA topic mixture. The Kullback-Leibler Divergence KLD $\left(s^{(j)}|s^{(j-d)}\right)$ measures surprise of speech at time $j$ given a speech $d$ steps away. Novelty at scale $w$ is the mean surprise of a central speech given speeches in a past window of $w$ steps. Transience is novelty under time reversal, measuring the mean surprise from the future. A rhetorically effective speech shifts current conversation to a new issue with a differing vocabulary, manifesting itself as a surprise asymmetry where novelty exceeds transience. We define this positive asymmetry as resonance (Eq. 5): the ability to break from the past and influence the future. An illustration of this asymmetry is shown in Figure 1c and in the central plot of Fig. 1 of the main text.

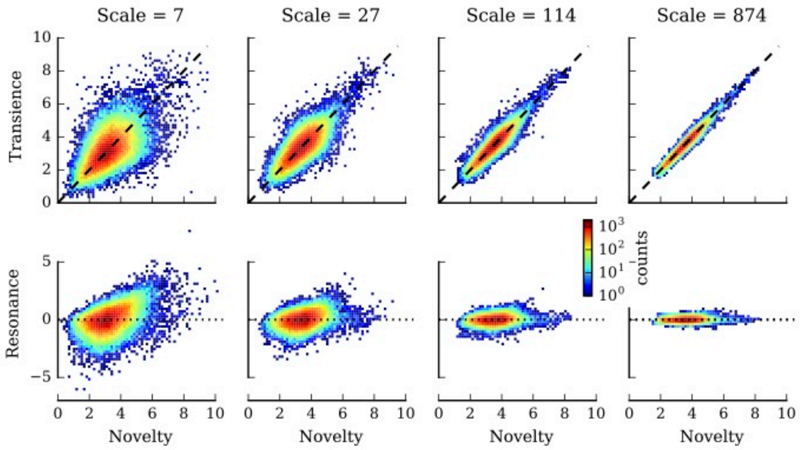


Figure 9: Density plots of transience v. novelty and resonance v. novelty for scales 7, 27, 114, and 874. Figure 1 uses density plots from scale 7, the first column in this figure.

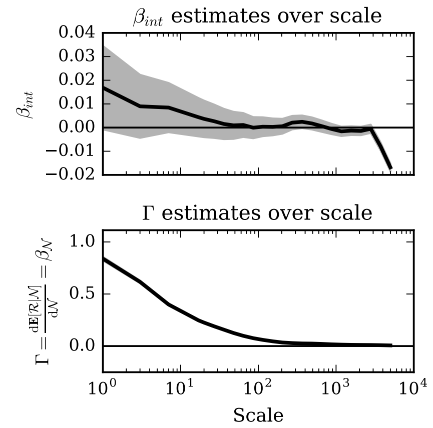


Figure 10: Parameter estimates from the model in Eq. 6, with 99% confidence intervals. $\Gamma = \frac{\mathrm{d}\mathbf{E}[\mathcal{R}|\mathcal{N}]}{\mathrm{d}\mathcal{N}}$ shows positive novelty bias from the smallest scales up to the mid-hundreds of speeches.

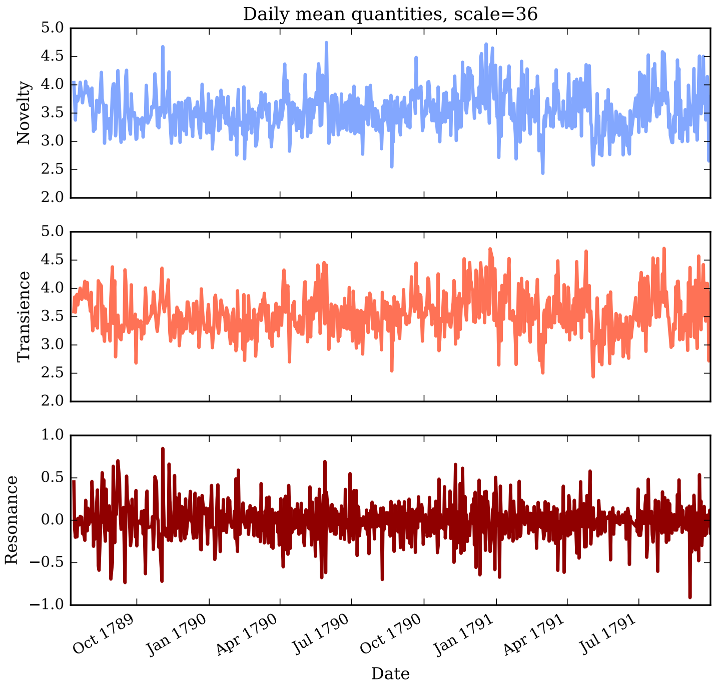


Figure 11: Daily bootstrap-corrected mean of novelty, transience, and resonance for the whole NCA period.

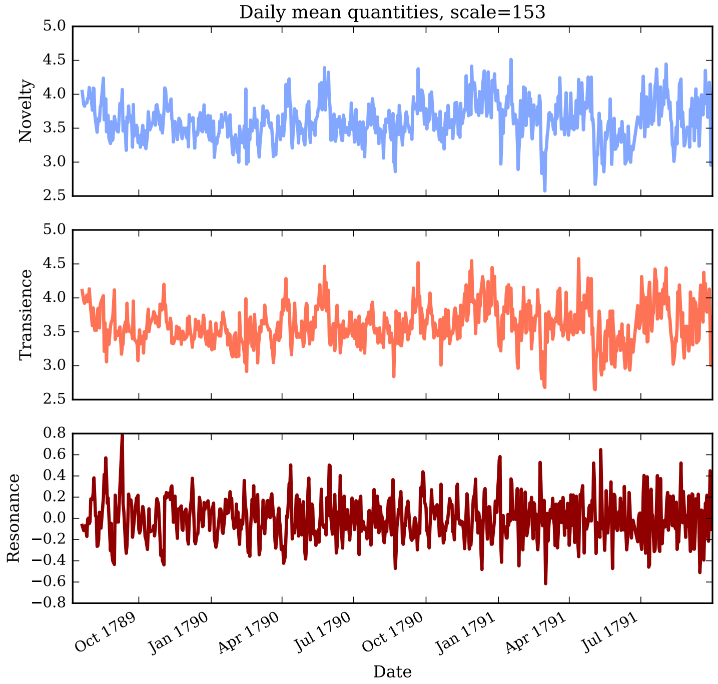


Figure 12: Daily mean of novelty, transience, and resonance as in Figure 11.

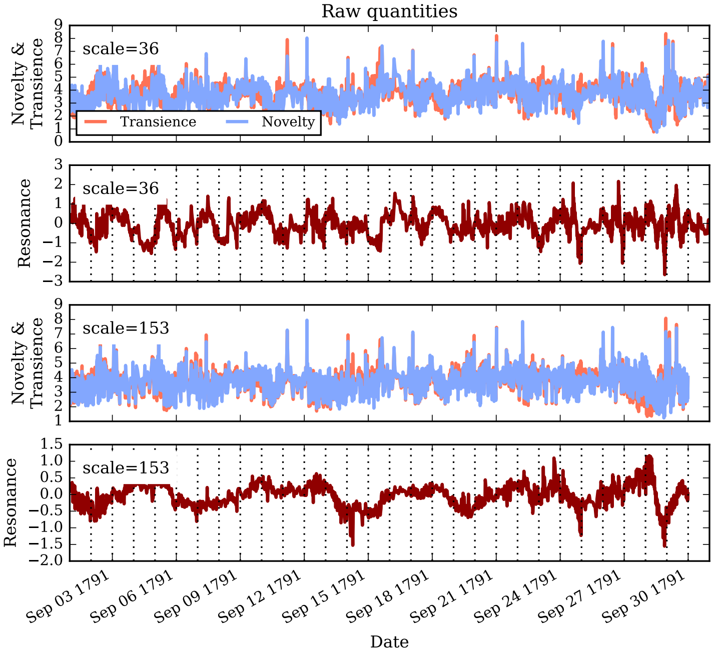


Figure 13: Comparison of raw resonance, novelty, and transience in September 1791, the last month of the NCA. Vertical lines in the resonance plots demarcate days. Note where excess transience over novelty produces low resonance, and vice versa. One can see daily patterns at scale 36, transitioning to multi-day patterns at scale 153. These patterns are exemplified in the power spectra of periodograms in Figure 16.

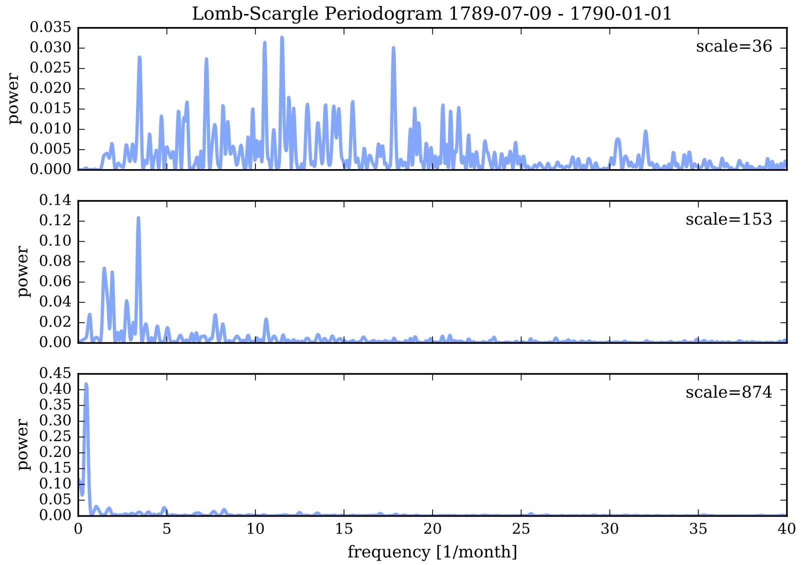


Figure 14: Lomb-Scargle periodograms for resonance at three scales for 1789, the first calendar year of the NCA.

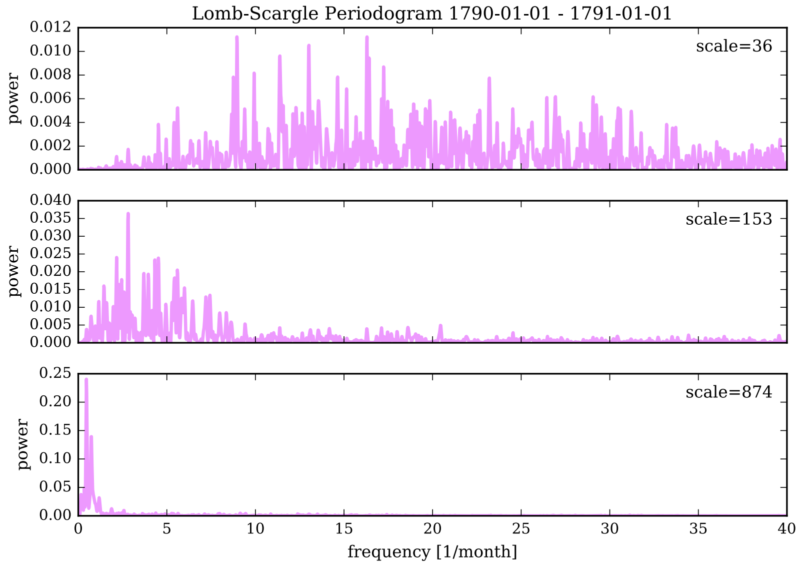


Figure 15: Lomb-Scargle periodograms for resonance at three scales for 1790.

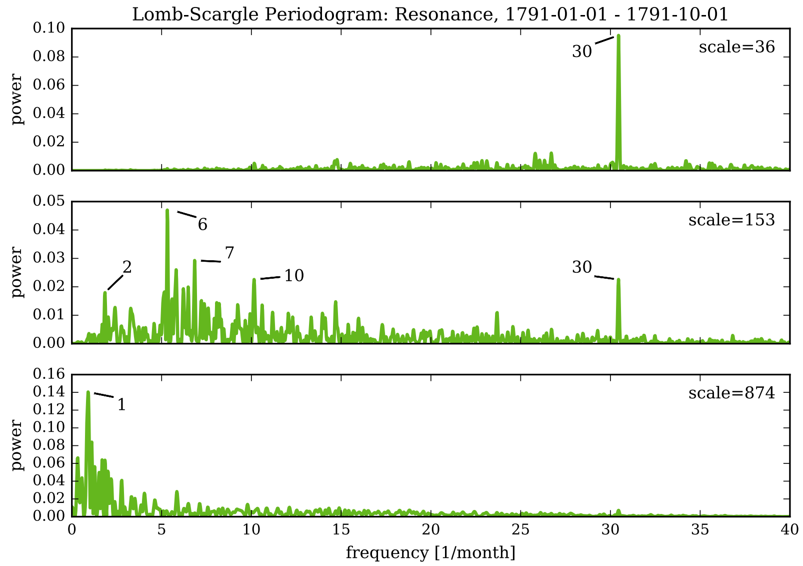


Figure 16: Lomb-Scargle periodograms for resonance at three scales for 1791, the final calendar year of the NCA.

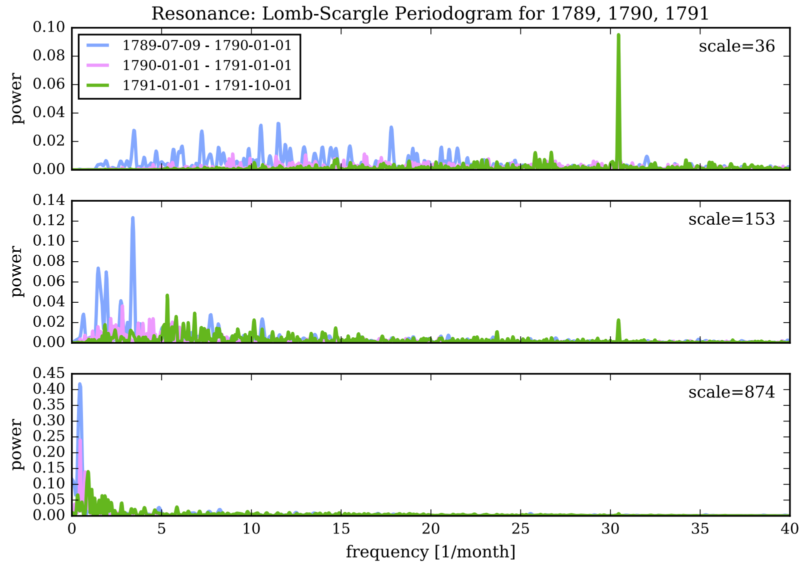


Figure 17: Lomb-Scargle periodograms for resonance at three scales: direct comparison for years 1789, 1790, 1791.

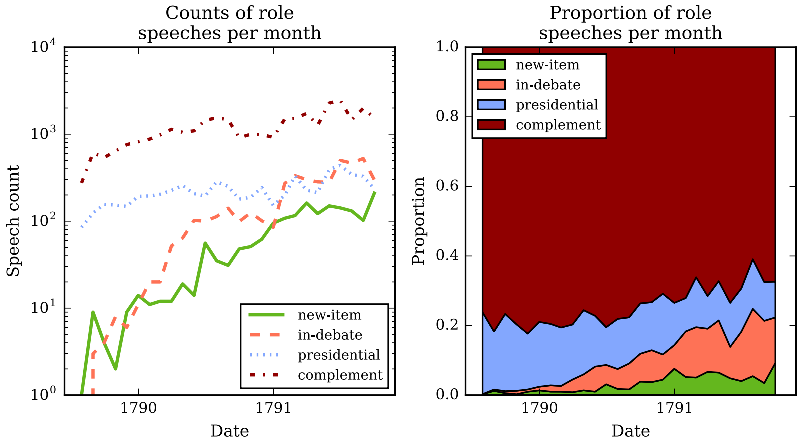


Figure 18: Monthly speech counts and proportion of the three organizational roles and their complement. As the NCA progresses, committee speech volume catches up to that of the president.

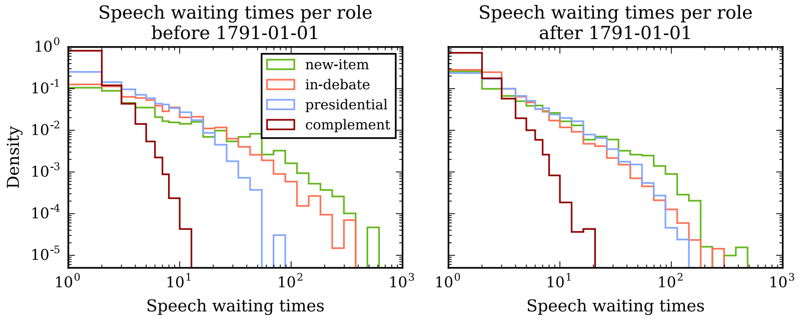


Figure 19: Waiting time distributions of the three organizational roles and their general speech complement. Pre-1791, the president is more regular than the committees. In 1791, the president's distribution is much more aligned with the committees', perhaps as a result of the committees' increased influence on debate rhythms.

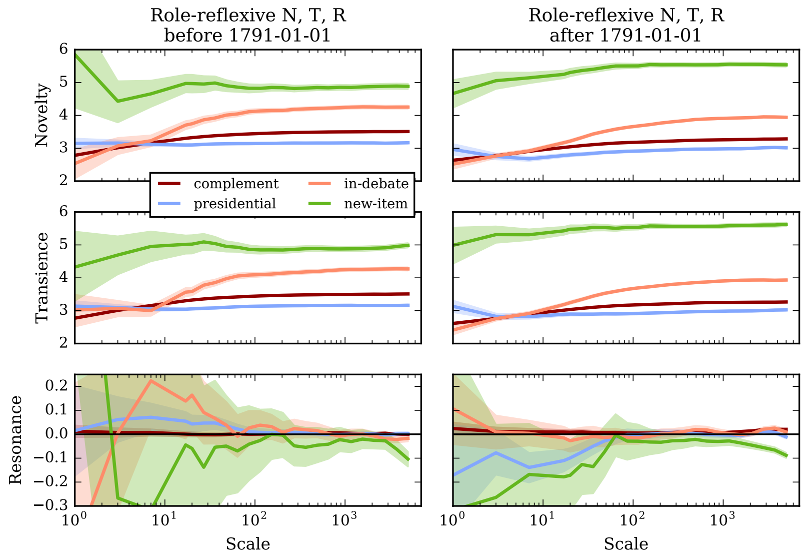


Figure 20: Mean reflexive novelty, transience, and resonance for each role, split into speeches before 1791-01-01 and after (columns 1 and 2), with 95% bootstrapped confidence intervals. "Reflexive" means that novelty, transience, and resonance are calculated using only speeches that match the center speech's role. So, a presidential speech is compared to only other presidential speeches, etc. Past scale 10, the president is the most similar to himself, even when compared to general speech, intuitively likely to be similar because of its serial nature in conversation.

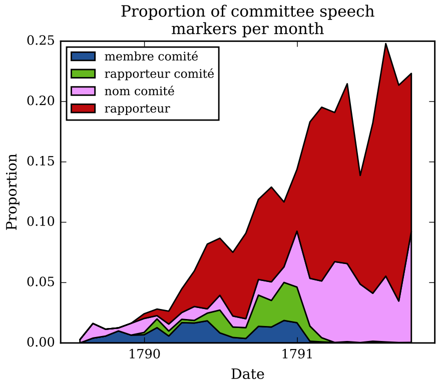


Figure 21: Monthly proportion of speeches containing each committee speech marker in Table 5.

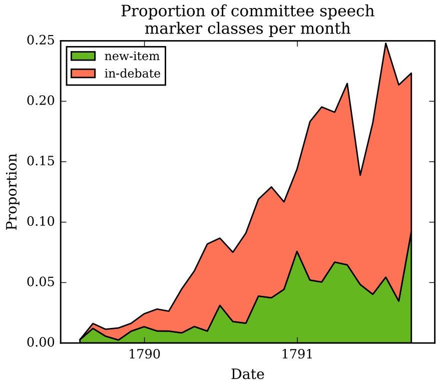


Figure 22: Monthly proportion of committee speech classes. Committee preamble assignment to class is shown in Table 7.

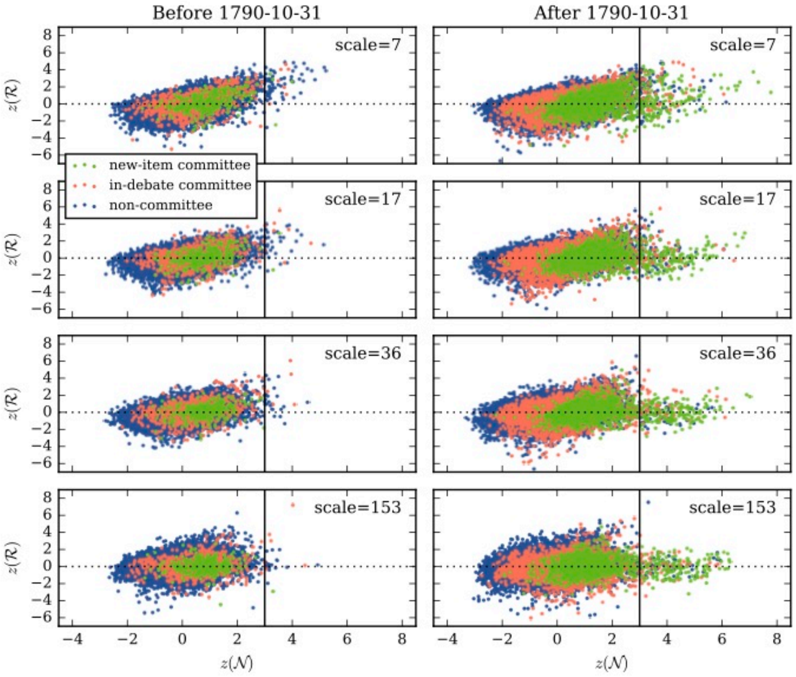


Figure 23: Scatter plots of resonance vs. novelty for several scales, split into new-item, in-debate, and non-committee speech. Each scale shows speeches before and after 1791-10-31, the epoch dividing point found for the scale range most sensitive to new-item committee effect on $\Gamma$ (see diachronic modeling appendix). The vertical line is a tail threshold marker of convenience, $z(\mathcal{N}) = 3$, for comparison between plots.

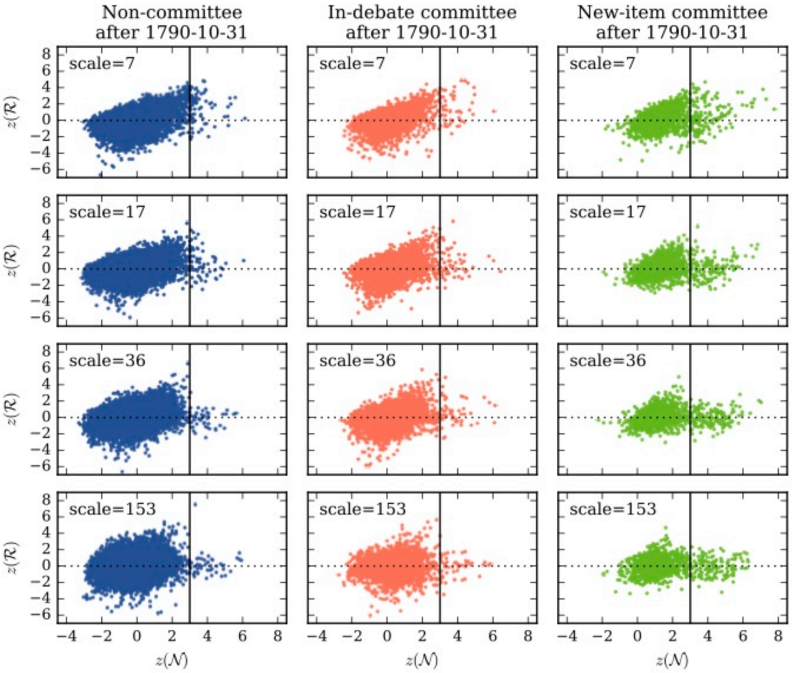


Figure 24: Scatter plots of resonance vs. novelty for only the second epoch, split by column into new-item, in-debate, and non-committee speech. One can see that the tail includes in-debate-rated and non-committee-rated speech. However, non-committee tail speeches tend to be misclassified by the regex search procedure and should be considered new-item (Table 9).

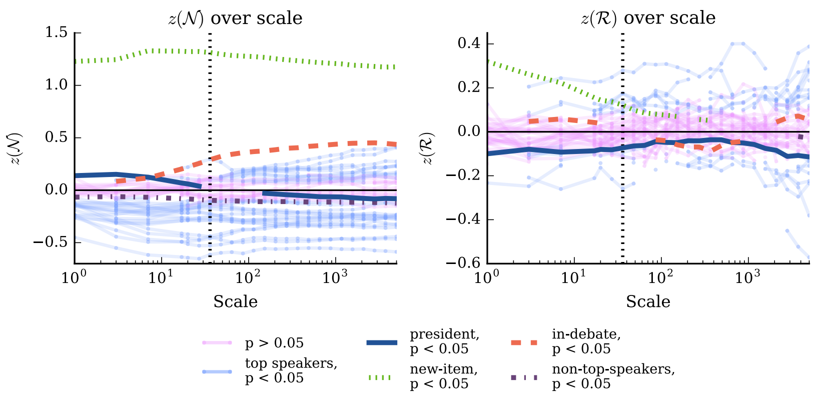


Figure 25: Traces of mean novelty and resonance for individuals and organizational roles over a range of scales. The outstanding novelty of new-item and in-debate committee proxies show committees' function as information injectors in the system. Coupled with high new-item resonance, committees fill the role of information injectors. The presidency enforces the agenda, obtaining above-average novelty (up to higher scale), but does not introduce information to be processed, accruing below-average resonance. The vertical line marks scale 36, where we profile individual entity and orator coefficients in Table 10.

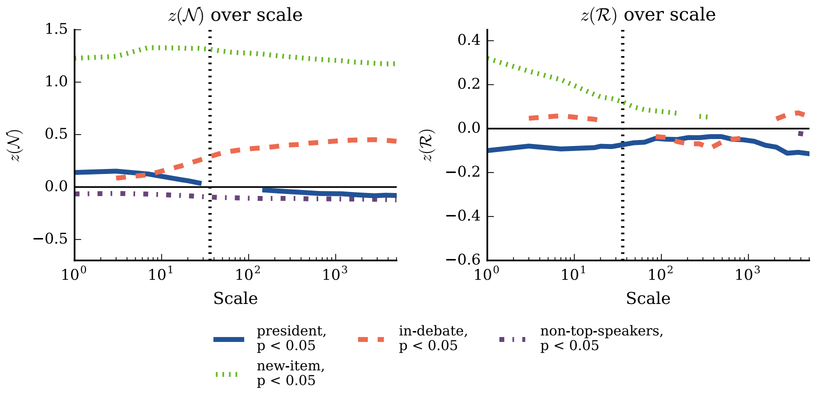


Figure 26: Plots as in Figure 25, showing only organizational roles and the trace for non-top-40 speakers.

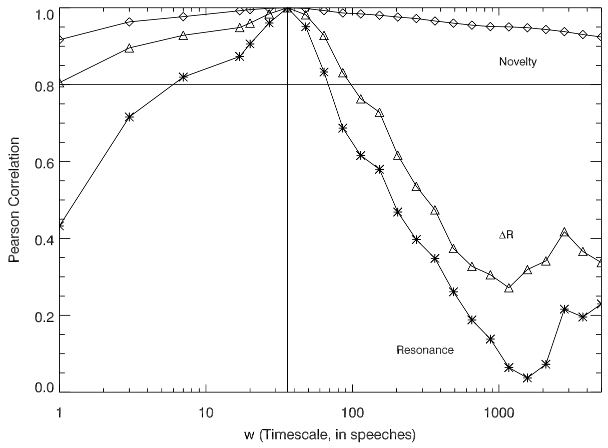


Figure 27: Pearson correlation between base timescale ($w = 36$) and wider ranges, for categories of Table 1 in main paper, for novelty, resonance, and $\Delta R$.

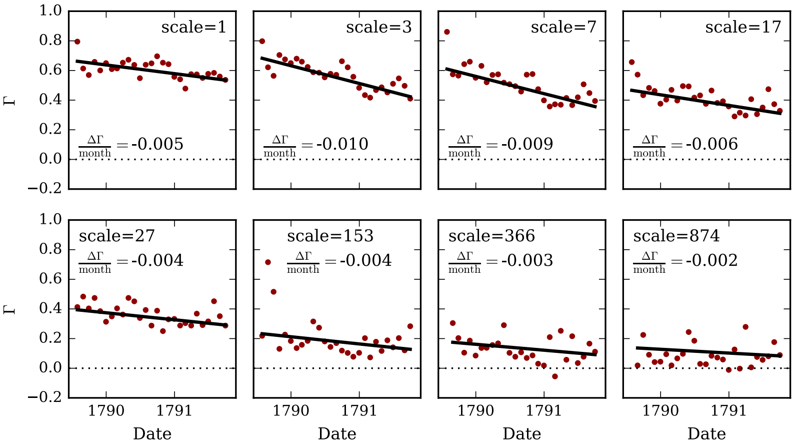


Figure 28: Novelty effectiveness $\Gamma(t) = \frac{\partial \mathbf{E}[\mathcal{R}|\mathcal{N},t]}{\partial \mathcal{N}}$ over a range of scales for the single epoch model. The trend line in each plot arises from including time interaction in the model of resonance and novelty (Eq. 9), producing the slope and intercept for $\Gamma(t)$. Each trend line is overlaid values of $\Gamma = \beta_{\mathcal{N}}$ produced from fitting Eq. 6 for speeches in each month. Note that the trend lines are not fits of the points in each plot. See Figure 29 for parameter estimates and confidence intervals of the model.

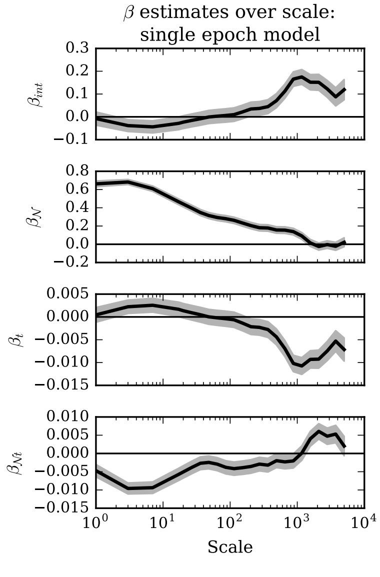


(a) parameter estimates

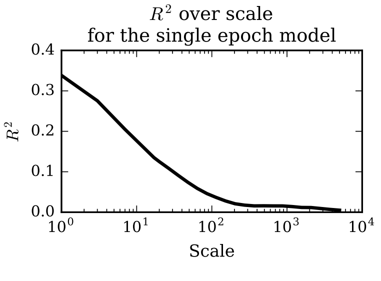


(b) $R^2$

Figure 29: Fitted parameter values with 99% confidence intervals and $R^2$ over scale for the single epoch model. $\beta_{\mathcal{N}t}$, the parameter representing the slopes in Figure 28, is negative for all scale with reasonable $R^2$.

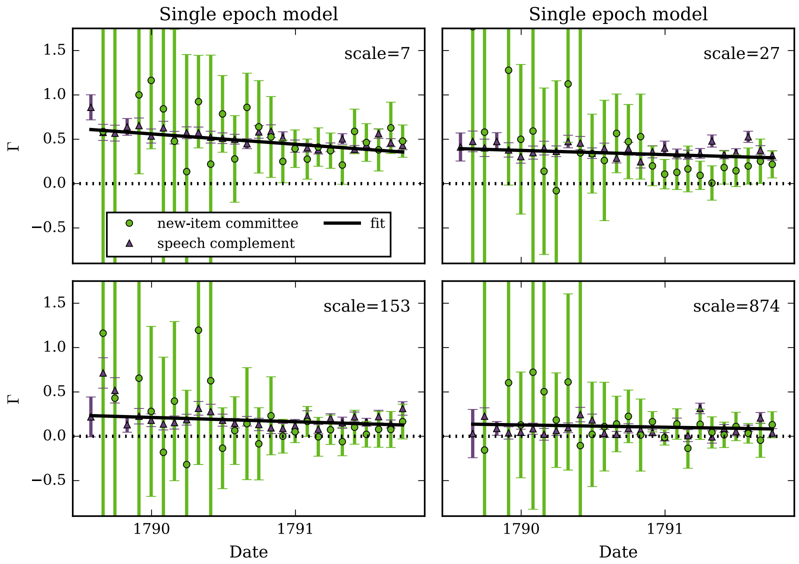


Figure 30: Monthly Γ behavior split between new-item committee and all other speech. Seen most clearly for scale 27 (upper right) the single epoch model cannot account for the drop in committees' novelty effectiveness during the final year.

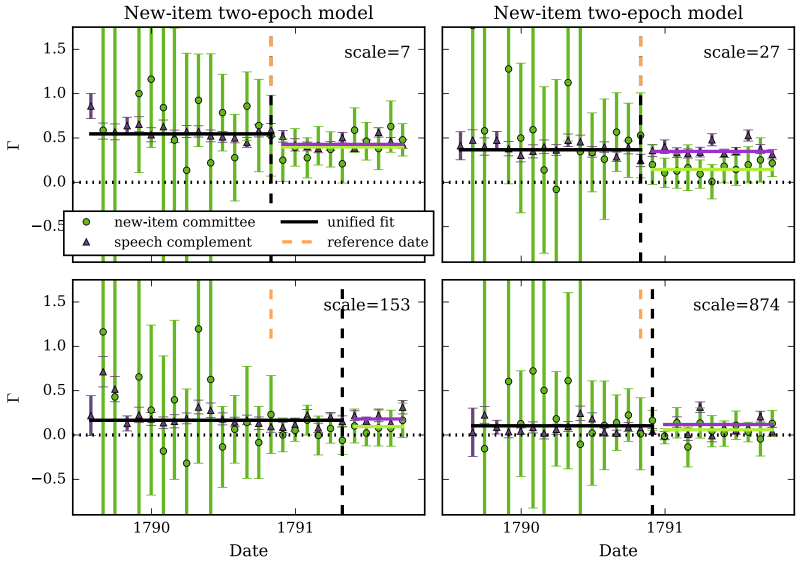


Figure 31: Monthly Γ behavior split between new-item committee and all other speech. In contrast to Figure 30, the new-item, two-epoch model captures the committees' drop in Γ. The reference divider, 1790-10-31, is used throughout the figures of this appendix.

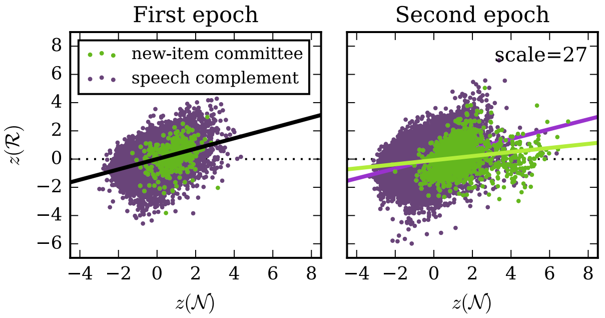


Figure 32: Fits of the new-item, two-epoch model for each epoch at scale 27. Parameters and $R^2$ over scale are shown in Figures 33 and 34.

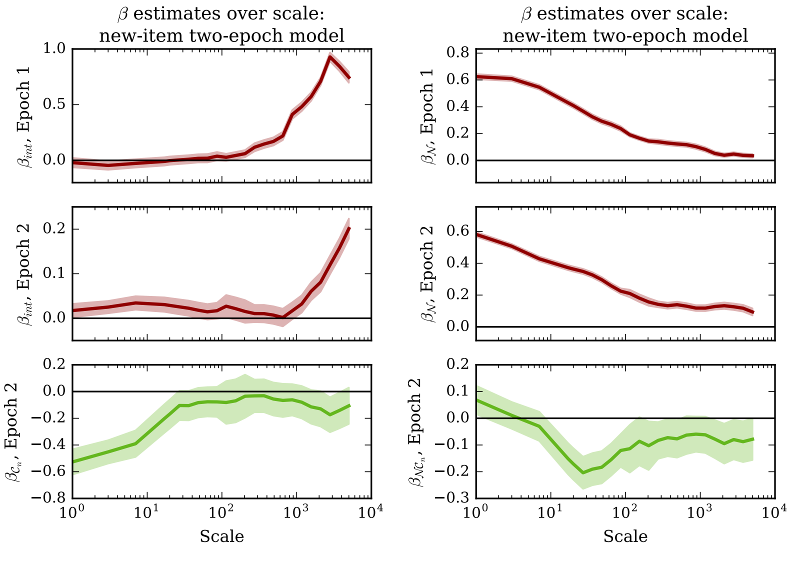


Figure 33: Fitted parameter values and 99% confidence intervals over scale for the new-item, two-epoch model.

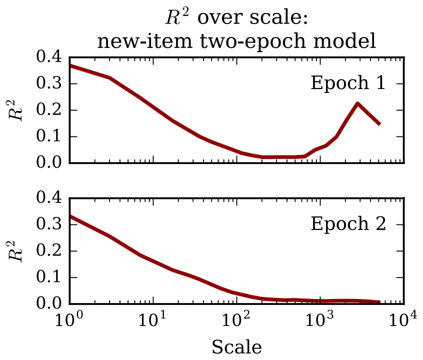


Figure 34: $R^2$ over scale for the new-item, two-epoch model.

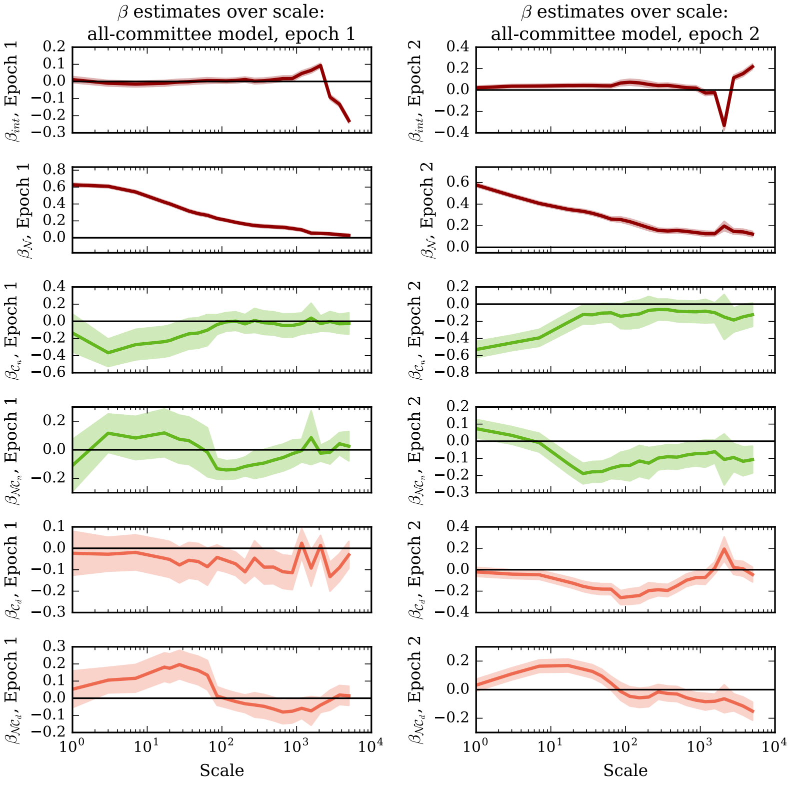


Figure 35: Fitted parameter values and 99% confidence intervals over scale for the all-commitee, two-epoch model.

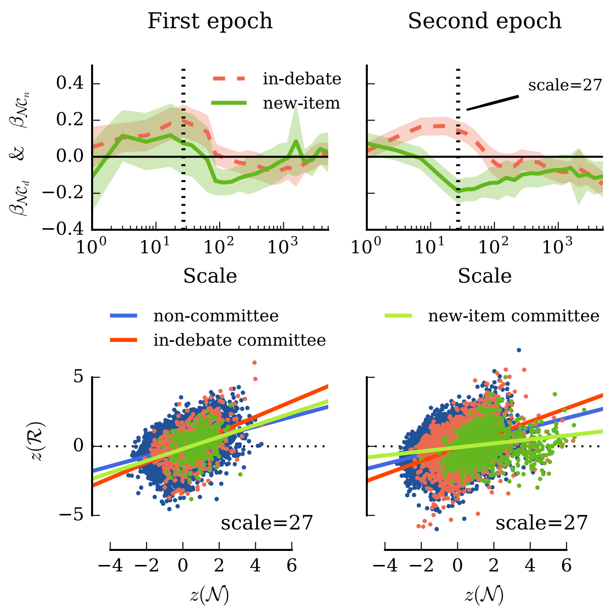


Figure 36: Slope parameters with 99% confidence intervals for the all-committee, two-epoch model over scale, with fits for each epoch at scale 27.

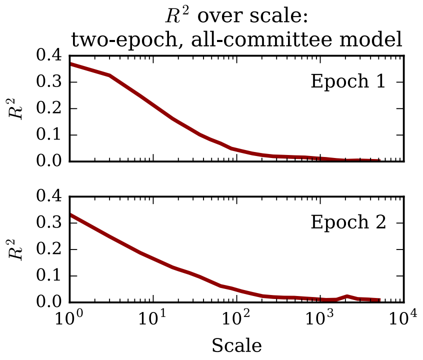


Figure 37: $R^2$ over scale for the all-committee, two-epoch model.

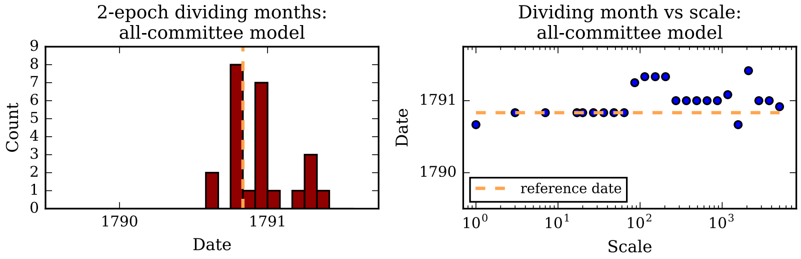


Figure 38: Epoch divider locations over scale for the all-committee, two-epoch model. At left, epoch division clusters around the end of 1790. At right, scales separate into contiguous zones of common partition. The reference divider for scales in the 10s of speeches, 1790-10-31, is useful when comparing this figure to Figure 31.

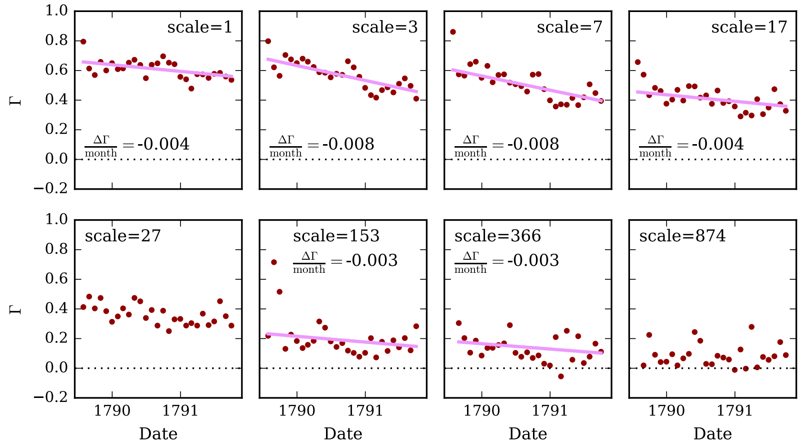


Figure 39: Novelty effectiveness $\Gamma(t) = \frac{\partial \mathbf{E}[\mathcal{R}|\mathcal{N},t]}{\partial \mathcal{N}}$ over a range of scales for the single epoch model, fit without new-item committee speech. Fit lines are not plotted if their associated $p > 0.05$. Note that the trend lines are not fits of the points in each plot. $\partial\Gamma/\partial t$ is comparitively higher than in Figure 28, to the point of non-significance at example scales 27 and 874.

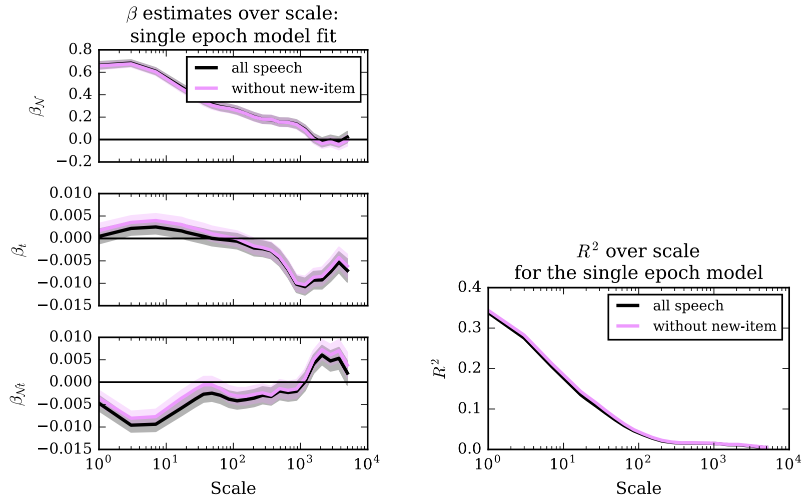


(a) parameter estimates

(b) $R^2$

Figure 40: Comparison of fitted parameter values with 99% confidence intervals and $R^2$ over scale for the single epoch model fit with and without new-item committee speech. $\partial\Gamma/\partial t = \beta_{\mathcal{N}t}$ is shifted higher over all scale.

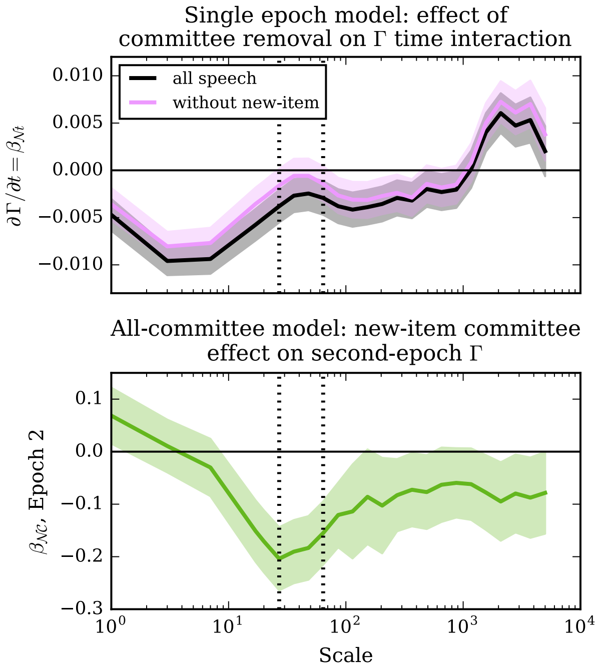


Figure 41: Explanation of decreasing Γ over time by epochal shift in new-item speech reception. $\partial\Gamma/\partial t = \beta_{\mathcal{N}t}$ for the NCA is shifted higher across scale when new-item committee speeches are removed. At scales between ∼20-60, marked by vertical lines, $\partial\Gamma/\partial t \approx 0$ after removal. Because this is the exact range of lowest Γ for new-item speech in the second epoch (bottom plot), the shift in new-item effectiveness is the reason for decreasing Γ over time in the single epoch model for that scale range.

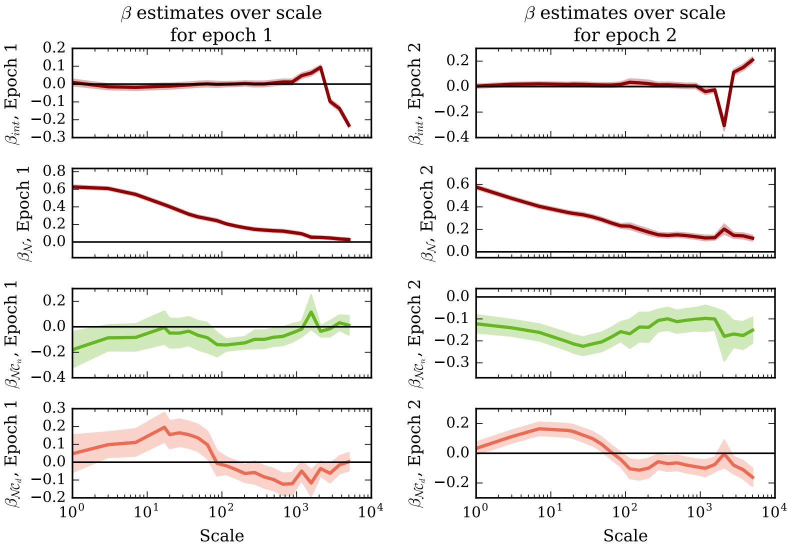


Figure 42: Fitted parameter values and 99% confidence intervals over scale for the all-committee, two-epoch, fixed intercept model.

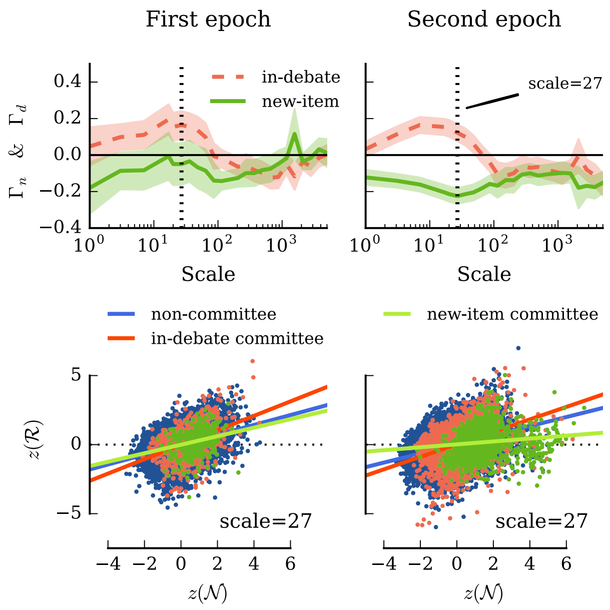


Figure 43: Slope parameters for the all-committee, two-epoch, fixed intercept model over scale, with fits for each epoch at scale 27. This is the plot presented in the main paper.

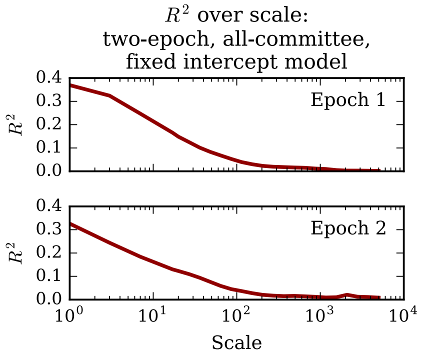


Figure 44: $R^2$ over scale for the all-committee, two-epoch, fixed intercept model.

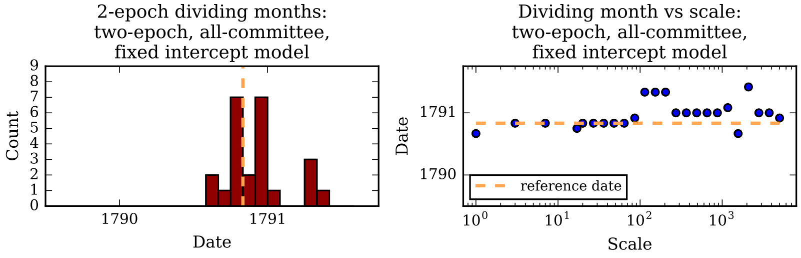


Figure 45: Epoch divider locations over scale for the all-committee, two-epoch, fixed intercept model. Results are comparable to those in Figure 38. The reference divider for scales in the 10s of speeches, 1790-10-31, is useful when comparing this figure to Figure 31.

## 7. Topic modeling

We coarse-grain each speech vector into a probability distribution over $K = 100$ semantic topics using Latent Dirichlet Allocation (LDA)[3]. Tables 13 through 17 contain the top 15 words by probability for every topic mixture.

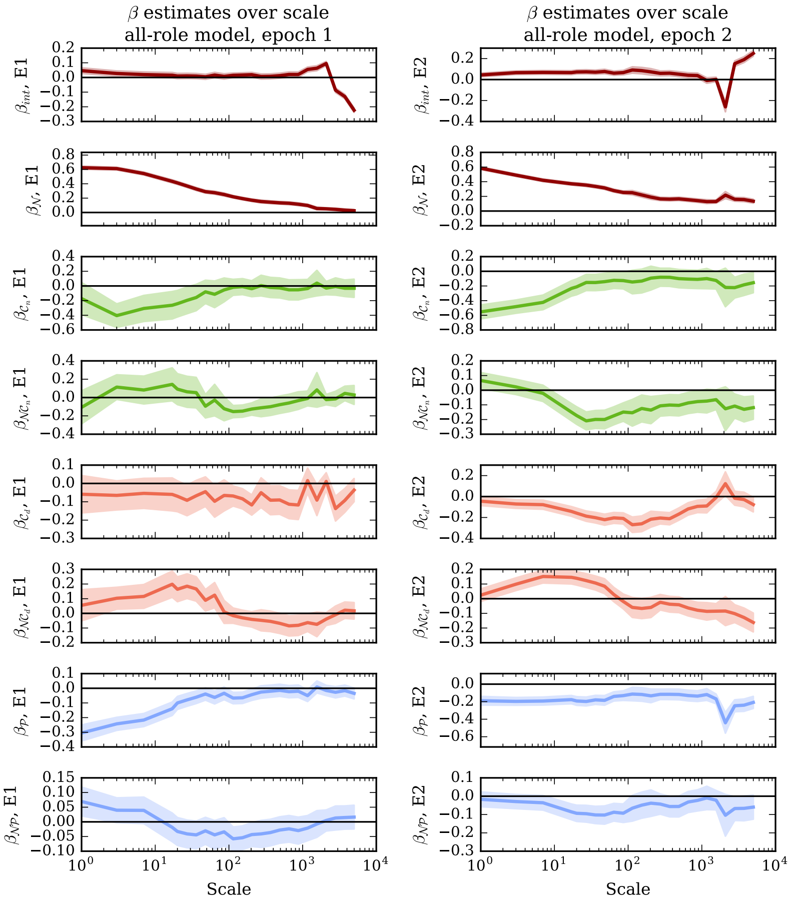


Figure 46: Fitted parameter values and 99% confidence intervals over scale for the all-role, two-epoch model.

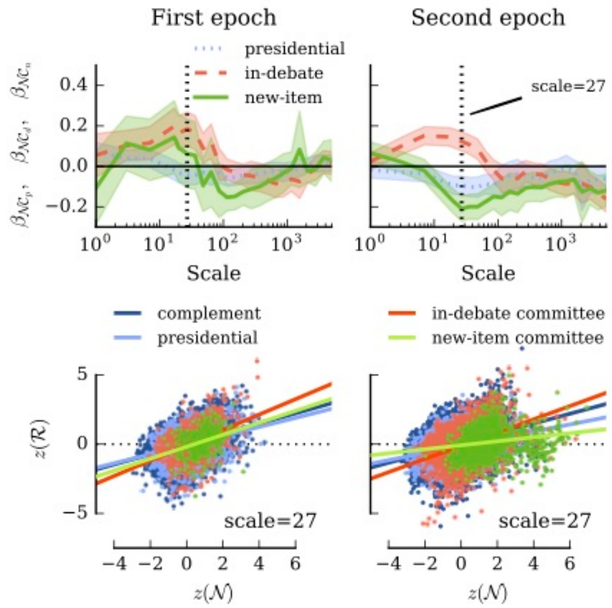


Figure 47: Slope parameters for the all-role, two-epoch model over scale, with fits for each epoch at scale 27.

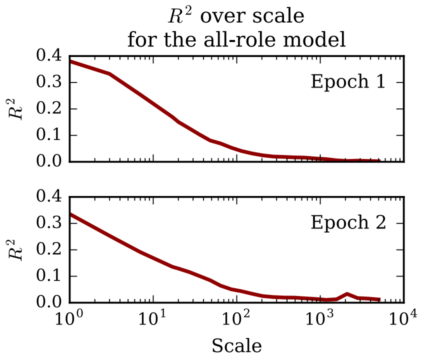


Figure 48: $R^2$ over scale for the all-role, two-epoch model.

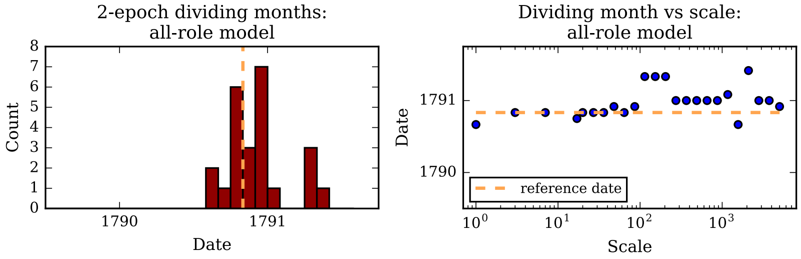


Figure 49: Epoch divider locations over scale for the all-role, two-epoch model. Results are comparable to those in Figure 38.

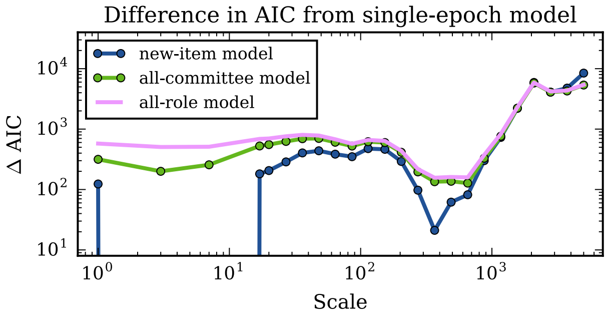


Figure 50: ΔAIC, the difference in AIC from the single epoch model to other models, over scale. Higher ΔAIC indicates the preferred model.

| 0 | 1 | 2 | 3 | 4 | 5 |
|---|---|---|---|---|---|
| cela | prisons | citoyens | églises | décret | criminelle |
| membre | accusation | avaient | etat | circonstances | deux |
| bien | prévôt | commandant | ecclésiastique | assurer | loi |
| messieurs | accusés | deux | revenus | nécessaires | dépositions |
| rires | faits | été | pauvres | toutes | preuves |
| demande | marseille | nîmes | propriétés | compte | procédure |
| voix | affaire | étaient | culte | rendre | juge |
| droite | décret | plus | été | exécution | juges |
| oui | assemblée | municipaux | propriété | moyens | accusation |
| plusieurs | été | garde | bénéfices | plus | jugement |
| non | comité | soldats | dîmes | prendre | fait |
| membres | nationale | municipalité | nation | commissaires | témoins |
| applaudissements | procédure | ville | ecclésiastiques | nationale | juré |
| gauche | tribunal | officiers | clergé | mesures | accusé |
| murmures | contre | régiment | biens | assemblée | jurés |
| 6 | 7 | 8 | 9 | 10 | 11 |
| corse | personne | procureurs | intérêt | peuples | diocèse |
| avignonais | nationale | entre | nombre | celui | ecclésiastiques |
| français | rendre | remplir | classe | tout | autorité |
| droits | après | commissaires | besoins | sous | civile |
| pays | demandé | public | bien | justice | culte |
| assemblée | fait | exercer | travail | encore | vicaires |
| peuple | garde | autres | tout | sans | ecclésiastique |
| pape | chez | exercice | moins | jamais | curé |
| ville | arrêté | publics | citoyens | grand | prêtres |
| réunion | assemblée | juges | toutes | lois | clergé |
| été | ordres | places | etat | peuple | eglise |
| comtat | paris | seront | encore | homme | curés |
| vœu | dit | tribunaux | nation | liberté | évêques |
| france | été | officiers | sans | hommes | évêque |
| avignon | roi | fonctions | plus | plus | religion |
| 12 | 13 | 14 | 15 | 16 | 17 |
| celle | desservie | toiles | villes | nation | ministres |
| été | ecclésiastique | celles | basrhin | fait | nations |
| non | succursale | sortie | nord | duc | étrangers |
| doivent | seront | livres | comité | droit | droit |
| autre | curé | étranger | électeurs | titre | affaires |
| toutes | art | entrée | assemblée | contrat | ministre |
| entre | directoire | royaume | cheflieu | droits | roi |
| autres | département | toutes | districts | france | traités |
| lois | district | seront | directoire | domaine | puissances |
| tout | cidevant | tarif | administrateurs | traité | nation |
| point | aura | autres | constitution | louis | français |
| loi | église | droit | ville | domaines | étrangères |
| plus | ville | quintal | district | prince | paix |
| elles | paroisses | marchandises | départements | été | france |
| même | paroisse | droits | département | roi | guerre |
| 18 | 19 | 20 | 21 | 22 | 23 |
| terre | bâtiments | royaume | amis | compter | septembre |
| sol | toulon | juifs | coupables | tenus | premier |
| terrains | ans | demande | moyens | desdits | août |
| après | concours | autres | toutes | sans | depuis |
| sans | grade | cidevant | révolution | pourront | décrets |
| marais | seront | député | loi | articles | novembre |
| terrain | port | été | publique | autres | avril |
| bois | etat | alsace | liberté | lesdits | juillet |
| droit | ports | assemblée | constitution | auront | octobre |
| mines | vaisseau | etats | sans | été | janvier |
| terres | mer | bretagne | ennemis | article | décembre |
| propriétés | service | pays | citoyens | présent | été |
| propriétaire | vaisseaux | députés | plus | décret | dernier |
| propriétaires | officiers | provinces | peuple | seront | mois |
| propriété | marine | province | contre | art | décret |

Table 13: Top 15 words of topics 1 through 23.

| 24 | 25 | 26 | 27 | 28 | 29 |
|---|---|---|---|---|---|
| annonce | fonds | conseil | matin | paru | assemblée |
| demie | dettes | municipalité | soir | avons | municipalités |
| matin | emprunt | été | demande | nom | habitants |
| jours | dette | municipalités | secrétaire | après | citoyens |
| assemblée | banque | administrateurs | donne | devoir | délibération |
| lève | intérêts | syndic | passe | présenter | général |
| congé | intérêt | procureur | hier | proposer | municipal |
| député | créanciers | districts | suite | cru | maire |
| demain | finances | administration | assemblée | projet | conseil |
| levée | escompte | avis | discussion | pensé | officiers |
| demande | rentes | général | lecture | décret | municipaux |
| soir | etat | directoires | procèsverbal | été | commune |
| trois | millions | directoire | séance | messieurs | paris |
| heures | billets | département | jour | comités | municipalité |
| séance | caisse | district | ordre | comité | ville |
| 30 | 31 | 32 | 33 | 34 | 35 |
| manière | nommer | suit | assemblées | plusieurs | annonce |
| avant | nombre | mis | partie | propose | membres |
| délibération | choix | entendu | coloniale | article | fauteuil |
| ajournement | plus | nom | état | ajournement | comte |
| point | suffrages | après | france | membres | été |
| moment | scrutin | suivant | générale | amendements | place |
| non | primaires | propose | libres | décrète | donné |
| décider | nomination | rapport | colons | voix | démission |
| questions | élections | adopté | hommes | délibérer | curé |
| agit | citoyens | décrète | décret | lieu | évêque |
| discussion | assemblée | projet | saintdomingue | assemblée | député |
| assemblée | élection | nationale | couleur | amendement | maury |
| demande | électeurs | assemblée | colonie | demande | président |
| savoir | membres | comité | assemblée | préalable | assemblée |
| question | assemblées | décret | colonies | question | abbé |
| 36 | 37 | 38 | 39 | 40 | 41 |
| adopté | royaume | car | seront | elles | prochaine |
| corps | tout | observation | projet | moment | ans |
| directoire | ecclésiastiques | quant | sciences | publique | pouvoir |
| administrés | civique | avis | ouvriers | toute | revision |
| bâtiments | décret | article | sous | même | constituant |
| rapport | fait | parce | administration | moyens | gouvernement |
| autorise | prêter | comité | paris | temps | constitutionnel |
| nationale | assemblée | paraît | académie | point | convention |
| emplacement | roi | cela | départements | intérêt | nationale |
| maison | fonctionnaires | pense | arts | enfin | législatures |
| département | prêté | préopinant | ouvrages | tout | vœu |
| district | publics | demande | chaussées | messieurs | nation |
| assemblée | constitution | très | ponts | sans | assemblée |
| décret | loi | serait | canal | toutes | législature |
| comité | serment | crois | travaux | plus | constitution |
| 42 | 43 | 44 | 45 | 46 | 47 |
| sommes | partie | soldat | payement | titre | poids |
| encore | dës | corps | acquéreurs | net | sols |
| besoins | qué | défense | adjudication | tit | valeur |
| comité | ëst | état | décret | ancienne | plus |
| somme | aussi | places | elles | mois | titre |
| état | point | service | baux | lieutenant | cloches |
| mois | dit | ministre | seront | secours | commission |
| dépense | quë | officiers | aliénation | régiment | sous |
| fonds | fait | soldats | ventes | capitaine | espèces |
| année | plus | hommes | prix | campagnes | cuivre |
| finances | lës | militaires | municipalités | art | pièces |
| public | lès | troupes | vente | services | argent |
| trésor | dès | guerre | domaines | pension | fabrication |
| dépenses | dés | militaire | nationaux | livres | monnaies |
| millions | lés | armée | biens | ans | monnaie |

Table 14: Top 15 words of topics 24 through 47.

| 48 | 49 | 50 | 51 | 52 | 53 |
|---|---|---|---|---|---|
| eût | elles | ici | plus | sans | décret |
| depuis | assemblées | moment | paris | propose | bien |
| devait | nombre | fait | augmentation | ordre | justice |
| dit | administration | pouvons | chaque | secours | dire |
| messieurs | département | encore | savoir | plus | pouvez |
| point | royaume | même | dépense | établissements | moment |
| pouvait | districts | bien | année | traitement | devez |
| alors | division | devons | sols | ordres | encore |
| après | assemblée | tout | jusqu | hôtel | serait |
| même | plus | été | total | maison | doute |
| fait | population | messieurs | frais | invalides | sans |
| fut | comité | plus | traitement | hôpitaux | plus |
| étaient | départements | sommes | liv | religieuses | aujourd |
| avaient | chaque | notre | somme | maisons | hui |
| été | villes | avons | livres | religieux | messieurs |

| 54 | 55 | 56 | 57 | 58 | 59 |
|---|---|---|---|---|---|
| chaque | mirabeau | papier | dettes | cas | titre |
| lieutenants | droite | inspecteurs | autres | chacun | suivants |
| compagnies | élève | sans | titulaires | même | conçu |
| infanterie | entendre | procèsverbaux | titre | plus | seront |
| plus | plusieurs | timbre | comité | articles | termes |
| sousofficiers | monsieur | générale | titres | toutes | donne |
| militaire | membres | autres | évaluation | titre | mis |
| seront | tribune | sous | officiers | après | projet |
| généraux | murmures | enregistrement | indemnité | pourront | voix |
| régiments | partie | droits | été | pourra | articles |
| service | parole | droit | prix | auront | lecture |
| corps | ordre | bois | finance | chaque | art |
| régiment | président | conservation | remboursement | aura | rapporteur |
| grade | assemblée | seront | offices | seront | adopté |
| officiers | demande | actes | liquidation | art | article |

| 60 | 61 | 62 | 63 | 64 | 65 |
|---|---|---|---|---|---|
| cents | france | décrète | particuliers | imprimé | rente |
| neuf | bonheur | arrêtés | bureaux | signé | dîme |
| sept | patriotisme | donner | administrateurs | faite | seigneur |
| dix | assemblée | sanction | administration | mention | rentes |
| huit | sentiments | été | publiques | écrit | propriétaire |
| cinq | citoyens | exécution | régisseurs | remis | seigneurs |
| six | nationale | ordres | droits | archives | été |
| trois | liberté | arrêté | généraux | commissaires | fief |
| quatre | notre | majesté | perception | assemblée | cas |
| deux | messieurs | décret | postes | bureau | indemnité |
| deniers | français | président | contributions | lettres | cidevant |
| mille | constitution | décrets | employés | pièces | rachat |
| sous | patrie | nationale | seront | procèsverbal | fonds |
| cent | nation | assemblée | receveurs | fait | droit |
| livres | plus | roi | régie | été | droits |

| 66 | 67 | 68 | 69 | 70 | 71 |
|---|---|---|---|---|---|
| aura | toutes | magistrats | commis | président | ledit |
| coupable | lois | toulouse | trésor | assister | estimée |
| puni | ordres | cour | dépenses | satisfaction | porte |
| crime | exécution | eaux | état | mention | autre |
| commis | ministère | metz | public | ordonne | maison |
| été | sous | rennes | nationale | paris | deux |
| délit | agents | rouen | général | répond | depuis |
| délits | responsabilité | arrêt | bureau | hommage | fait |
| mort | fonctions | bordeaux | trésorerie | procèsverbal | ladite |
| tout | roi | vacations | comptabilité | séance | paris |
| cas | exécutif | paris | commissaires | députation | sieurs |
| peines | administration | bailliage | extraordinaire | barre | celle |
| loi | ministres | offices | compte | fait | rue |
| contre | pouvoir | chambre | comptes | nationale | jusqu |
| peine | ministre | parlement | caisse | assemblée | sieur |

Table 15: Top 15 words of topics 48 through 71.

| 72 | 73 | 74 | 75 | 76 | 77 |
|---|---|---|---|---|---|
| perception | année | laquelle | présenté | faite | aller |
| produit | contribuables | suis | organisation | soient | nominal |
| villes | répartition | très | présenter | décrétée | motion |
| gabelle | revenus | donner | objet | amendement | appel |
| culture | livre | ministre | propose | mise | demandent |
| droit | raison | etc | décret | angély | ajournement |
| sel | rôles | honneur | discussion | propose | fermée |
| impôts | chaque | fait | rapport | saintjeand | parole |
| provinces | contributions | signé | assemblée | voix | priorité |
| plus | impôt | lecture | constitution | assemblée | plusieurs |
| prix | foncière | nationale | travail | appuie | membres |
| millions | imposition | monsieur | plan | adoptée | assemblée |
| droits | revenu | président | articles | proposition | voix |
| tabac | impositions | assemblée | projet | demande | demande |
| impôt | contribution | lettre | comité | motion | discussion |

| 78 | 79 | 80 | 81 | 82 | 83 |
|---|---|---|---|---|---|
| contre | rien | même | peu | nombre | public |
| nationaux | autre | aucun | état | celle | sans |
| commerce | crois | fonctions | quelques | quatrième | déclaration |
| dette | dire | lieu | jours | après | principes |
| livres | plus | sans | nombre | second | tout |
| monnaie | fait | cas | plusieurs | plus | lois |
| valeur | messieurs | pouvoir | même | autre | constitution |
| plus | demande | législature | fait | partie | société |
| émission | dit | pourra | été | premier | homme |
| millions | parce | décret | moment | troisième | citoyen |
| circulation | tout | membres | temps | trois | citoyens |
| papier | très | administratifs | depuis | classe | liberté |
| numéraire | car | roi | très | seconde | droit |
| argent | cela | législatif | encore | première | loi |
| assignats | bien | corps | plus | deux | droits |

| 84 | 85 | 86 | 87 | 88 | 89 |
|---|---|---|---|---|---|
| état | sceaux | articles | contre | manière | intérêt |
| gratifications | autorise | décret | tenu | assemblée | négociants |
| liste | celui | ceuxci | justice | dernier | notre |
| ans | patentes | premier | après | domaines | royaume |
| traitements | lettres | décrété | devant | aliénation | français |
| secours | roi | ajouter | acte | état | étranger |
| services | proclamation | mot | commissaire | comité | agriculture |
| après | décrets | disposition | paix | mai | industrie |
| décret | mois | rapporteur | officier | biens | marchandises |
| service | relatif | rédaction | tribunal | nationaux | ports |
| personnes | concernant | mots | juge | département | compagnie |
| traitement | portant | demande | pourra | même | inde |
| pension | jour | amendement | lieu | municipalité | manufactures |
| été | même | propose | cas | décret | france |
| pensions | décret | article | police | celle | commerce |

| 90 | 91 | 92 | 93 | 94 | 95 |
|---|---|---|---|---|---|
| renvoie | volonté | devoir | seront | fait | dispositions |
| finances | législatif | dire | elles | principes | mère |
| pétition | gouvernement | été | corps | comment | royaume |
| renvoyée | liberté | honneur | service | parce | parents |
| membre | lois | crois | ordre | droit | plus |
| compte | loi | tout | armes | cela | roi |
| constitution | représentants | avais | ligne | sans | régent |
| affaire | pouvoirs | bien | publique | non | fils |
| rapports | exécutif | plus | troupes | question | biens |
| rapport | constitution | messieurs | force | dire | régence |
| comités | droit | assemblée | citoyens | plus | loi |
| renvoi | peuple | moi | nationale | quand | droit |
| assemblée | nation | suis | garde | point | père |
| demande | roi | mes | nationales | bien | enfants |
| comité | pouvoir | mon | gardes | dit | famille |

Table 16: Top 15 words of topics 72 through 95.

| 96 | 97 | 98 | 99 |
|---|---|---|---|
| charge | affaires | bien | plus |
| madame | seront | grand | celle |
| ladite | jugements | aussi | même |
| chambre | judiciaire | nombre | don |
| faites | parties | seraient | district |
| veuve | district | moyen | communauté |
| femme | justice | peu | adhésion |
| tailleur | paix | autre | adresses |
| marchand | juge | celui | fait |
| cidevant | appel | aurait | patriotique |
| compter | jugement | pourrait | décrets |
| intérêts | cassation | moins | nationale |
| roi | tribunaux | même | assemblée |
| somme | tribunal | serait | ville |
| livres | juges | plus | adresse |

Table 17: Top 15 words of topics 96 through 99.

[1] B. D. Jones, F. R. Baumgartner, The politics of attention: How government prioritizes problems, University of Chicago Press, Chicago, IL, USA, 2005.

[2] J. G. Foster, A. Rzhetsky, J. A. Evans, Tradition and innovation in scientists' research strategies, American Sociological Review 80 (5) (2015) 875–908.

[3] D. M. Blei, A. Y. Ng, M. I. Jordan, Latent Dirichlet allocation, Journal of Machine Learning Research (JMLR) 3 (2003) 993–1022.

[4] J. Murdock, C. Allen, S. DeDeo, Exploration and exploitation of Victorian science in Darwin's reading notebooks, Cognition 159 (2017) 117–126.

[5] W. L. Benoit, M. J. Smythe, Rhetorical theory as message reception: A cognitive response approach to rhetorical theory and criticism, Communication Studies 54 (1) (2003) 96–114.

[6] R. A. Harris, Reception studies in the rhetoric of science, Technical Communication Quarterly 14 (3) (2005) 249–255.

[7] M. Foucault, Power/Knowledge: Selected interviews and other writings, 1972–1977, Pantheon, New York, NY, USA, 1980.

[8] C. Danescu-Niculescu-Mizil, L. Lee, B. Pang, J. Kleinberg, Echoes of power: Language effects and power differences in social interaction, in: Proceedings of the 21st international conference on World Wide Web, ACM, 2012, pp. 699–708.

[9] S. Klingenstein, T. Hitchcock, S. DeDeo, The civilizing process in London's Old Bailey, Proceedings of the National Academy of Sciences 111 (26) (2014) 9419–9424. arXiv:http://www.pnas.org/content/111/26/9419.full.pdf.

[10] M. M. Bakhtin, The dialogic imagination: Four essays, University of Texas Press, Austin, TX, USA, 2010.

[11] R. A. Blythe, W. Croft, S-curves and the mechanisms of propagation in language change, Language 88 (2) (2012) 269–304.

[12] S. Kullback, R. Leibler, On information and sufficiency, Annals of Mathematical Statistics 22 (1) (1951) 79–86.

[13] L. Itti, P. Baldi, Bayesian surprise attracts human attention, Vision Research 49 (10) (2009) 1295–1306.

[14] T. Tackett, Becoming a Revolutionary, Princeton University Press, Princeton, NJ, USA, 2014.

[15] W. H. Sewell, Historical events as transformations of structures: Inventing revolution at the Bastille, Theory and society 25 (6) (1996) 841–881.

[16] K. M. Baker, Inventing the French Revolution: essays on French political culture in the eighteenth century, Cambridge University Press, Cambridge, UK, 1990.

[17] K. M. Baker, D. Edelstein, Scripting revolution: a historical approach to the comparative study of revolutions, Stanford University Press, Stanford, CA, USA, 2015.

[18] W. F. Buckley Jr., Our mission statement, National Review 1.

[19] D. P. Baron, Legislative organization with informational committees, American Journal of Political Science 44 (3) (2000) 485–505.

[20] K. A. Shepsle, B. R. Weingast, Positive theories of Congressional institutions, Legislative Studies Quarterly 19 (2) (1994) 149–179.

[21] N. R. Lomb, Least-squares frequency analysis of unequally spaced data, Astrophysics and Space Science 39 (2) (1976) 447–462.

[22] J. D. Scargle, Studies in astronomical time series analysis. II-Statistical aspects of spectral analysis of unevenly spaced data, The Astrophysical Journal 263 (1982) 835–853.

[23] S. DeDeo, D. Krakauer, J. Flack, Evidence of strategic periodicities in collective conflict dynamics, Journal of The Royal Society Interface (2011) rsif20100687.
